# Supplementary material for: SAVE: Spectral-Shift-Aware Adaptation of Image Diffusion Models for Text-driven Video Editing
Source: arXiv:2305.18670 source file (2023-12-01)
Supplement: Supplementary file 1 [file X_suppl.tex]

\clearpage
\setcounter{page}{1}
\maketitlesupplementary

\section{Overview}
The supplementary material has been organized into the following sections:
\begin{itemize}
    \item Section~\ref{sec:preliminary}: Preliminaries
    \item Section~\ref{ex_details}: Experimental Details
    \item Section~\ref{sec:them_proof}: Proof of Theorem
    \item Section~\ref{sec:motivation}: More on Spectral Shift Optimization
    \item Section~\ref{algo}: SAVE Algorithm
    \item Section~\ref{additional_results}: Additional Results
     \item Section~\ref{userstudy}: User Study Details
     \item Section~\ref{zero-shot}: Zero-Shot Text-to-Video Generation
     \item Section~\ref{sec:attention}: Exploring Attention for Video Editing
     \item Section~\ref{sec:discussion}: Discussion and Limitations
\end{itemize}
% \vspace{-5mm}
We have also attached the following:
\begin{itemize}
    \item Additional supporting results (comparison, attention maps, etc.) can be found in the PPT file \textbf{\emph{"Additional-Supporting-Results.pptx"}}
    \item Example edited videos can be found in \textbf{\emph{"Edited-Example-Videos.zip"}} folder.
    \item PyTorch implementation of our method can be found in the attached \textbf{\emph{"SAVE-Code.zip".}} folder
\end{itemize}

\section{Preliminaries}\label{sec:preliminary}
\paragraph{DDIM Sampling and Inversion.} During inference, we apply deterministic DDIM sampling~\cite{ddim} to convert a random noise $z_T$ to a clean latent $z_0$ with the help of trained diffusion model ($\theta$):
\begin{equation}\label{eq:ddim_sampling}
\begin{split}
    z_{t-1} = \sqrt{\alpha_{t-1}}\left(\frac{z_t - \sqrt{1-\alpha_t}\epsilon_{\theta}(z_t)}{\sqrt{\alpha_t}}\right) + 
    \sqrt{1-\alpha_{t-1}}\epsilon_{\theta}(z_t), \\ \quad t=T,\ldots,1, 
\end{split}
\end{equation}
where $\alpha_t = \prod_{i=1}^{t}(1-\beta_i)$ is a parameter for noise scheduling~\cite{ddim, ddpm}. DDIM Inversion is the reverse process of DDIM sampling where we can map a clean latent $z_0$ to a noisy latent $\hat{z}_T$:
\begin{equation}\label{eq:ddim_inversion}
\begin{split}
    \hat{z}_{t} = \sqrt{\alpha_{t}}\left(\frac{\hat{z}_{t-1} - \sqrt{1-\alpha_{t-1}}\epsilon_{\theta}(\hat{z}_{t-1})}{\sqrt{\alpha_{t-1}}}\right) + \\
    \sqrt{1-\alpha_{t-1}}\epsilon_{\theta}(\hat{z}_{t-1}), \quad t=T,\ldots,1, 
\end{split}
\end{equation}
For applying DDIM inversion to a video, we invert each frame of the input video to the noise space. To reconstruct the original latent space using $\mathcal{P}$, we set the classifier-free guidance scale $s_{cfg}$ to 1. 

\paragraph{Low-Rank Adaptation (LoRA).} builds on the insight: pre-trained language models, despite being projected to a smaller subspace, possess a low "intrinsic dimension" and retain efficient learning capabilities. This insight led to the intuition that weight updates during adaptation also possess a low "intrinsic rank." To constrain the update of a pre-trained weight matrix $W_0\in \mathbb{R}^{d\times k}$, LoRA decompose it as $W_0+\Delta W=W_0+BA$, where $B\in \mathbb{R}^{d\times r}, A\in \mathbb{R}^{r\times k}$, and the rank $r \ll \min(d,k)$.
During training, $W_0$ remains static without receiving gradient updates, while $A$ and $B$ contain trainable parameters.

Both $W_0$ and $\Delta W=BA$ are applied to the same input, and their respective output vectors are combined coordinate-wise. For $h = W_0x$, the revised forward pass equation becomes:
\begin{equation}
h = W_0 x + \Delta W x = W_0 x + BA x
\label{eq:lora}
\end{equation}
Additional details can be found in the original LoRA paper.

\section{Experimental Details}\label{ex_details}
In Table~\ref{tab:overview}, we show a simple comparison with baseline methods. Unlike CogVideo~\cite{hong2022cogvideo} and MAV~\cite{singer2023makeavideo}, we do not train the model from scratch. Compared to SOTA, our proposed method has more functionalities (e.g. Zero-Shot capabilities) with approximately 100$\times$ less tunable parameters.   

For training, we employ Adam optimizer with betas 0.9 and 0.999 and a weight decay of 5e-3. We take F(=12) frames where each frame has a resolution of $512\times512$.  We use a guidance scale, $s_{cfg}$ of 7.5 for video editing. 

\begin{table*}[t!]
    \centering    
    \caption{\textbf{A simple comparison with SOTA benchmarks}. Our proposed method reduces the tunable parameters by almost 100$\times$. \textit{SAVE} is also compatible for \textit{Zero-shot} text-to-video generation without any tuning. Here, CogVideo~\cite{hong2022cogvideo} and MAV~\cite{singer2023makeavideo} consider training a T2V model from scratch before using it for generation during inference. Also, Text2LIVE~\cite{text2live} trains an image generator from scratch. Therefore, the term "tuning" is not applicable (N/A) to them.}
    \scalebox{0.95}{
    \begin{tabular}{c|c|c|c|c|c|c}
        \toprule
        \textbf{Method} & CogVideo~\cite{hong2022cogvideo} & MAV~\cite{singer2023makeavideo} & Text2LIVE~\cite{text2live} & TAV~\cite{wu2022tune} & Video-P2P~\cite{liu2023video} & \textit{SAVE} (Ours)    \\
        \midrule
        Full Training & $\checkmark$ & $\checkmark$ & $\checkmark$ &$\times$  &$\times$ & $\times$ \\
        Zero-Shot & $\checkmark$ & $\checkmark$ & $\times$ & $\times$ & $\times$  & $\checkmark$ \\
        $\#$Tunable Params & N/A & N/A & N/A & 24M & 24M & \textbf{0.2M} \\
        \bottomrule
    \end{tabular}}
    \vspace{2mm}
    \vspace{-2mm}
    \label{tab:overview}
\end{table*}
\begin{figure*}[h!]
%\begin{center}
\centering
%\hspace{-5mm}
%\begin{minipage}{0.35\textwidth}
    \includegraphics[width=0.7\linewidth, trim={0cm 0cm 0cm 0cm}]{./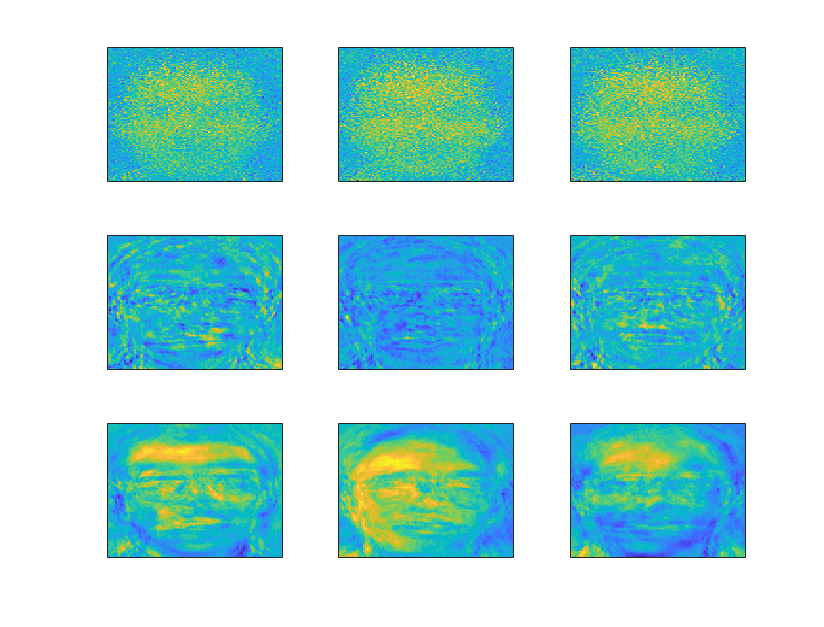}
%    \end{center}
    \vspace{-2mm}
    \caption{\footnotesize{The \textbf{impact of generating random samples in the spectral domain and adapting spectral coefficients to statistics of the real samples}. \textit{First row}: generating random noise for each pixel according to the mean and variance of original samples. \textit{Second row}: combining spectral components of the original data with random coefficients. \textit{Third row}: randomly combined spectral components according to mean and variance of spectral coefficients of the real data. } }
\label{fig:lgn} 
\end{figure*}

\begin{figure*}[htb!]
%\begin{center}
\centering
%\hspace{-5mm}
%\begin{minipage}{0.35\textwidth}
    \includegraphics[width=0.85\linewidth, trim={0cm 0cm 0cm 0cm}]{./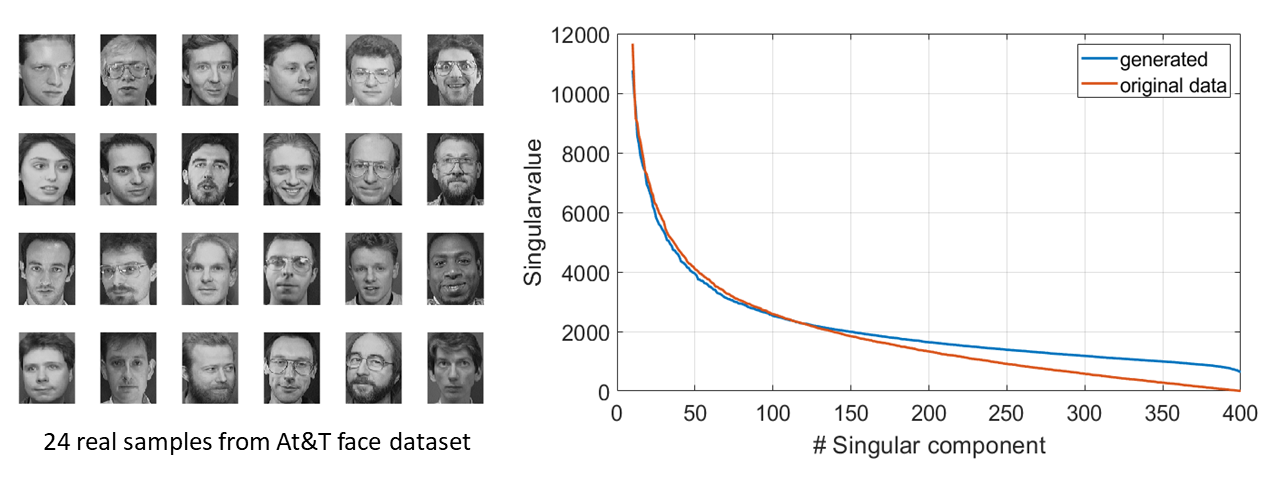}
%    \end{center}
    \caption{\footnotesize{ \textbf{A set of samples from AT\&T dataset and the distribution of singular values}. Regularizing the generated samples restricts main spectral components to follow the spectrum of original data while it allows small singular values to deviate more from the original spectrum in order to span fine details. } }
\label{fig:att_svs}
\vspace{10pt}
\end{figure*}

\begin{figure*}[t!]
%\begin{center}
\centering
%\hspace{-5mm}
%\begin{minipage}{0.35\textwidth}
    \includegraphics[width=0.95\linewidth]{figs/Regularizer_effect.pdf}
%    \end{center}
    \caption{\footnotesize{\textbf{Impact of our proposed regularizer illustrated through attention maps.} With the use of the regularizer, the generated cross-attention (CA) maps are more compact and on point. This gives us the fine-matching ability shown by the special token attention. The proposed regularizer keeps the special token's attention from being spread out any further than the coarse class token. For example, the word yellow should only affect the animal area, not other regions. Zoom in for better visibility. }}
\label{fig:effect_regularizer}
\end{figure*}

\begin{figure*}[t!]
%\begin{center}
\centering
%\hspace{-5mm}
%\begin{minipage}{0.35\textwidth}
    \includegraphics[width=0.95\linewidth]{figs/More_reg_effect.pdf}
%    \end{center}
    \caption{\footnotesize{\textbf{Additional attention maps visualization to show the impact of our proposed regularizer.}  The attention maps show that the regularizer is on point in terms of region-wise editing effects. These results also show the capabilities of SAVE in handling diverse command prompts. Zoom in for better visibility. }}
\label{fig:additiona_eefect_regular}
\end{figure*}

\setlength{\textfloatsep}{7pt}
\begin{algorithm*}[htb]

% \SetAlgoLined
 \caption{\textbf{\textit{SAVE}} Video Editing} \label{alg:attention}
\textbf{Input:} A source prompt $\mathcal{P}$ and a source video $X$ with $F$ frames.\\
\textbf{Output:} An editing prompt $\mathcal{P}^*$ and edited video $X^{*}$.\\
\textbf{Parameter:} Number of timesteps $T$, Number of attention layers $L$, Number of iterations $K$\\
\textbf{Fine-tuning:}  \tcp*{We first perform the fine-tuning} \\
 Obtain clean latents using the encoder, $z_0^f = \mathcal{E}(X); f = 1 \ldots F$ \\
 Forward diffusion process for noisy latents, $z_t = \{z_t^{f}; f = 1 \ldots F\}  \hspace{1mm} \text{where} \hspace{1mm} t = 1 \ldots T$      \tcp*{Gradually add noise to the clean latents} \\
 Inflated T2V model ($\theta$) initialized from Stable Diffusion (SD) T2I model ($\theta_I$) \\ 
 % Latent features from DDIM inversion: $[z_{T}]$;\\
 % $z_{T}^* \gets z_{T}$; \\
 $\boldsymbol{W}^{Q}_i = \boldsymbol{U_i}\boldsymbol{\Sigma_i} \boldsymbol{V_i}^T$; $i=1 \ldots L$ \hspace{1mm} \text{where} \hspace{1mm} $\Sigma_i=\text{diag}(\sigma_i)$  \tcp*{Spectral decomposition of query matrices } \\ 
 Initialize Spectral Shift Parameter, $\delta_i = \text{Zeros}(P); P= \text{size}(\Sigma_i)$  \tcp*{Singular value differences} \\
 $\boldsymbol{\Sigma}_i^{\delta_i} = \text{diag}(\text{ReLU}(\sigma_i+\delta_i))$  \tcp*{New updated formulation of $\Sigma_i$} \\
 % Initialized unconditional embedding $\varnothing^*$ and optimized unconditional embedding $\varnothing$;\\
 Total spectral shift $\delta = [\delta_1, \delta_2, ..., \delta_L]$ \tcp*{For all attention layers} \\
 \For{$k=1,2, \ldots, K$}{
     $t\sim \text{Uniform}(\{1 \ldots T\})$  \tcp*{For Timestep Embedding} \\
     $\varepsilon\sim\mathcal{N}(0,I)$    \tcp*{Noise Sampling} \\
     $\mathcal{L}(\delta) &= E_{z_0}\left\|\varepsilon-\varepsilon_{\theta_{\delta}}\left(z_t, t, p \right)\right\|_2^2
     +\lambda\mathcal{L}_{r}(\delta)$  \tcp*{Calculate Loss} \\
    Update $\delta$ using $\nabla_{\theta} \mathcal{L}(\delta)$ \\
    % $z_{t-1}, M_{t} \gets DM(z_{t},\mathcal{P},t, \varnothing)$\;
    % $M_{t}^* \gets DM(z_{t}^*,\mathcal{P}^*,t, \varnothing^*)$\;
    % $\widehat{M}_{t} \gets Edit(M_{t}, M_{t}^*, t)$\;
    % $z_{t-1}^* \gets DM(z_{t}^*,\mathcal{P}^*,t,\varnothing^*)\{M_{t}^* \gets \widehat{M}_{t}\}$\;
    % $\alpha \leftarrow B\big(\overline{M}_{t, w}\big) \cup B\big(\overline{M}_{t, w^*}^*\big)$\;
    % $z_{t-1}^* \leftarrow(1-\alpha) \odot z_{t-1}+\alpha \odot z_{t-1}^*$\;
 }
  Fine-tuned model $\hat{\theta}$ \\

\textbf{Inference:} \\
Set T= 50, $s_{cfg}=7.5$ \tcp*{Number of inference steps} \\
DDIM Inversion of $X$ to obtain $z_T$ \\
\For{$t=T, T-1, \ldots 1$}{ 
       $ z_{t-1} = \sqrt{\alpha_{t-1}}\left(\frac{z_t - \sqrt{1-\alpha_t}\epsilon_{\hat{\theta}}(z_t)}{\sqrt{\alpha_t}}\right) + 
    \sqrt{1-\alpha_{t-1}}\epsilon_{\hat{\theta}}(z_t)$
}
\textbf{Return} $X^{*} = \mathcal{D}(z_0)$

\end{algorithm*}
\section{Proof of Theorem 1}\label{sec:them_proof}
% \textcolor{cyan}{MOHSEN, Please put the proof for Theorem 1. }
Eigenvalues of a diagonal matrix are equal to diagonal elements. However, in the case of non-diagonal matrices, non-diagonal elements deviate eigenvalues from the diagonal elements. According to the Gershgorin circle theorem \cite{weisstein2003gershgorin}, eigenvalues of a square matrix are bounded within a circle with the center at the $n^{\text{th}}$ diagonal element and the radius is the absolute summation of non-diagonal elements at the $n^{\text{th}}$ column. Thus, in order to find a bound for each eigenvalue, it is sufficient to find a bound for the absolute summation of non-diagonal elements of that matrix.

Let $\boldsymbol{USV}^T$ show SVD of $\boldsymbol{D}$ and $\boldsymbol{U}\boldsymbol{\Sigma}_g\boldsymbol{V}^T$ point to decomposition of $\boldsymbol{D}_g$ in terms of singular vectors of $\boldsymbol{D}$. Spectral coefficients of $\boldsymbol{D}$ and Spectral coefficients of $\boldsymbol{D}_g$ are defined as $\boldsymbol{C}=\boldsymbol{U}^T\boldsymbol{D}$ and $\boldsymbol{C}_g=\boldsymbol{U}^T\boldsymbol{D}_g$. Since $\boldsymbol{U}$ is a unitary matrix, singular values of $\boldsymbol{D}$ are equal to singular values of $\boldsymbol{C}$ and singular values of $\boldsymbol{D}_g$ is equal to those of $\boldsymbol{C}_g$. 

Singular values of $\boldsymbol{C}_g$ are equal to the square root of eigenvalues of $\boldsymbol{C}_g^T\boldsymbol{C}_g$. 

According to the definition of $\boldsymbol{C}_g$, the diagonal elements of $\boldsymbol{C}_g^T\boldsymbol{C}_g$ is $N(m_n^2+2m_nx_n+x_n^2)$. In which, $m_n$ is the mean of the $n^{\text{th}}$ spectral coefficient and $x_n$ is a deviation with variance $v_n$. Similarly a non-diagonal element at the $(i,n)$ entry is equal to $N(m_im_n+m_ix_n+m_nx_i+x_i_x_n)$. Expected values of non-diagonal entries of $\boldsymbol{C}_g^T\boldsymbol{C}_g$ will be:
$$
E[\boldsymbol{C}_g^T\boldsymbol{C}_g]=[a_{i,n}]\n
$$
$$
a_{i,n}=Nm_im_n
$$
Summation of non-diagonal elements of the $n^{\txet{th}}$ column is equal to $Nm_n\sum_{i\ne n}m_i$. This summation is an upper bound for the deviation the $n^{\txet{th}}$  eigenvalue.
Mean and variance of $\boldsymbol{C}_g$ entries are coming from the mean and variance of the original spectral coefficients $\boldsymbol{C}$. In other words, $\boldsymbol{C}$ is a sample from a random matrix, $\boldsymbol{C}_g$. Thus, the $n^{\text{th}}$ eigenvalue of $\boldsymbol{C}$ lies within the same circle as $\boldsymbol{C}_g$. The maximum distance between Eigenvalues of $\boldsymbol{C}$ and $\boldsymbol{C}_g$ will be 2 times of the corresponding Greshgorin circle.
$$
|\sigma_n^2(D)-\sigma_n^2(D_g)| \le 2 Nm_n\sum_{i\ne n}m_i
$$
$$
|\sigma_n(D)-\sigma_n(D_g)| \le  \frac{2Nm_n\sum_{i\ne n}m_i}{\sigma_n(D)+\sigma_n(D_g)}
$$

\begin{figure*}[h!]
%\begin{center}
\centering
%\hspace{-5mm}
%\begin{minipage}{0.35\textwidth}
    \includegraphics[width=1\linewidth, trim={0cm 0cm 0cm 0cm}]{./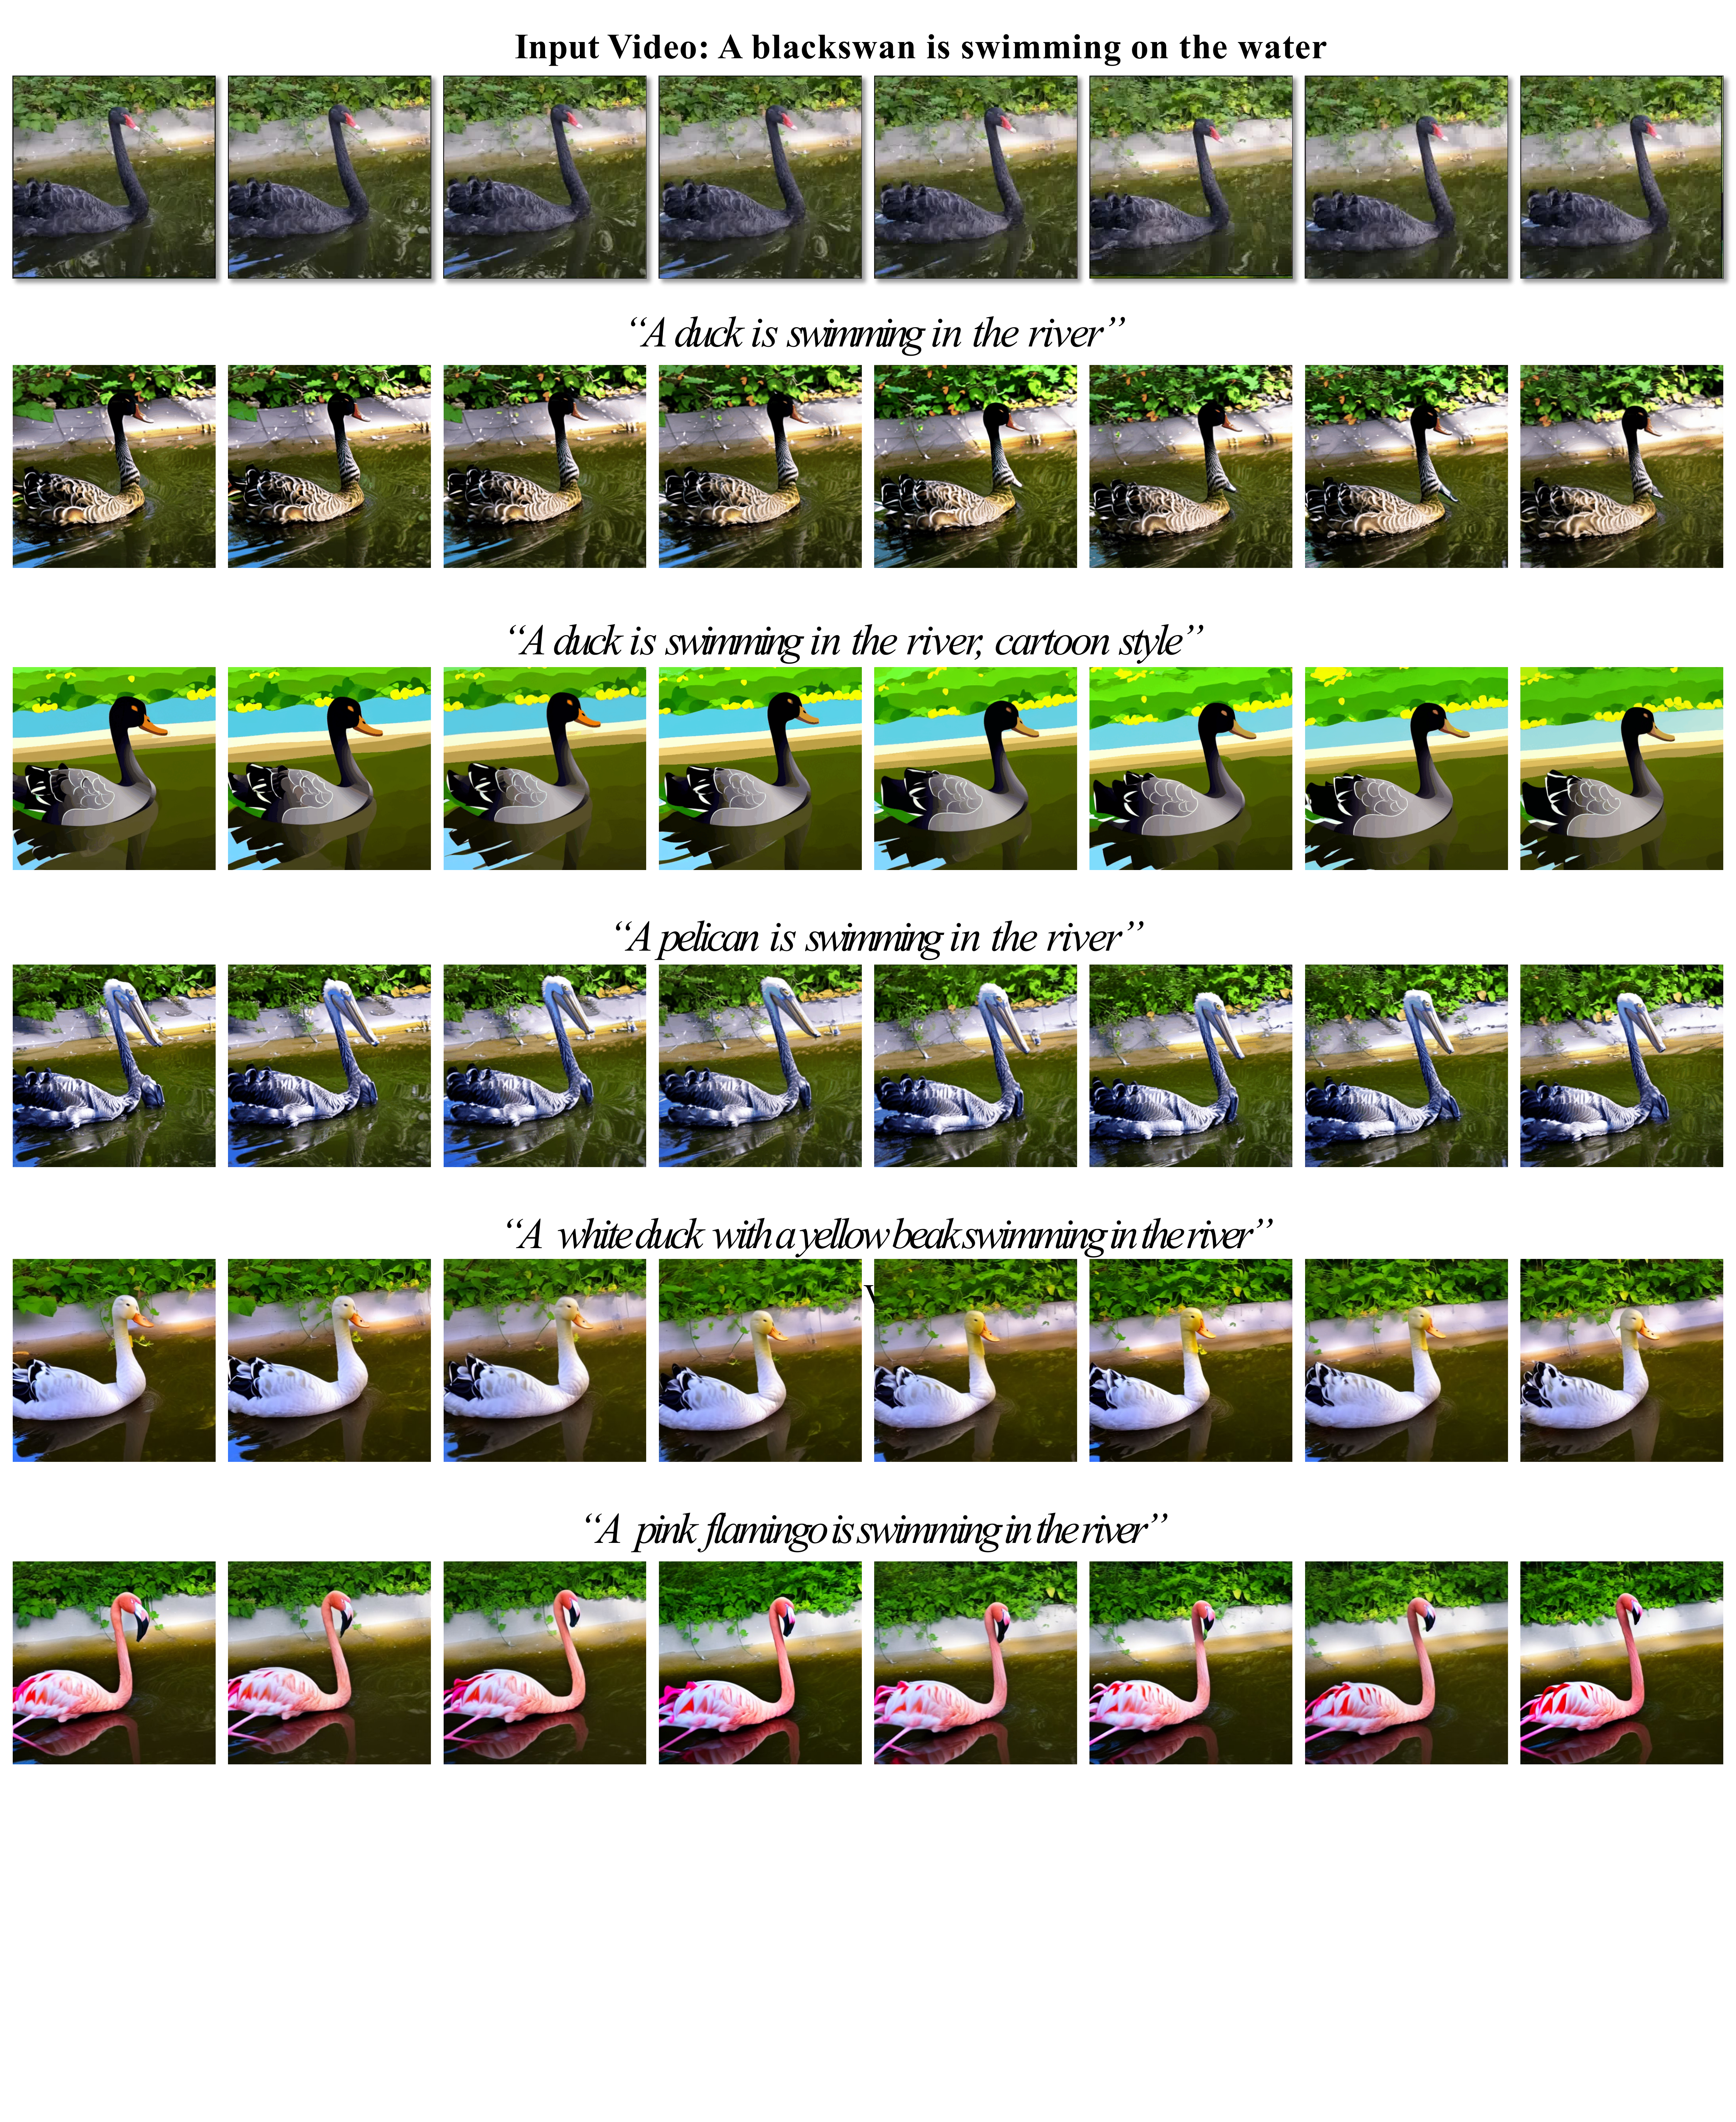}
%    \end{center}
    \caption{\footnotesize{\textbf{Shape editing results} of our method. The first row shows the frames of the input video. In the second row, the input video has been edited based on the prompt, and "swan" is replaced with "duck". Similarly, the shape of the object has been successfully edited and conditioned on the input prompt in the subsequent rows. Zoom in for better visibility. } }
\label{fig:swan_1}

\end{figure*}
\begin{figure*}[t!]
%\begin{center}
\centering
%\hspace{-5mm}
%\begin{minipage}{0.35\textwidth}
    \includegraphics[width=1\linewidth, trim={0cm 0cm 0cm 0cm}]{./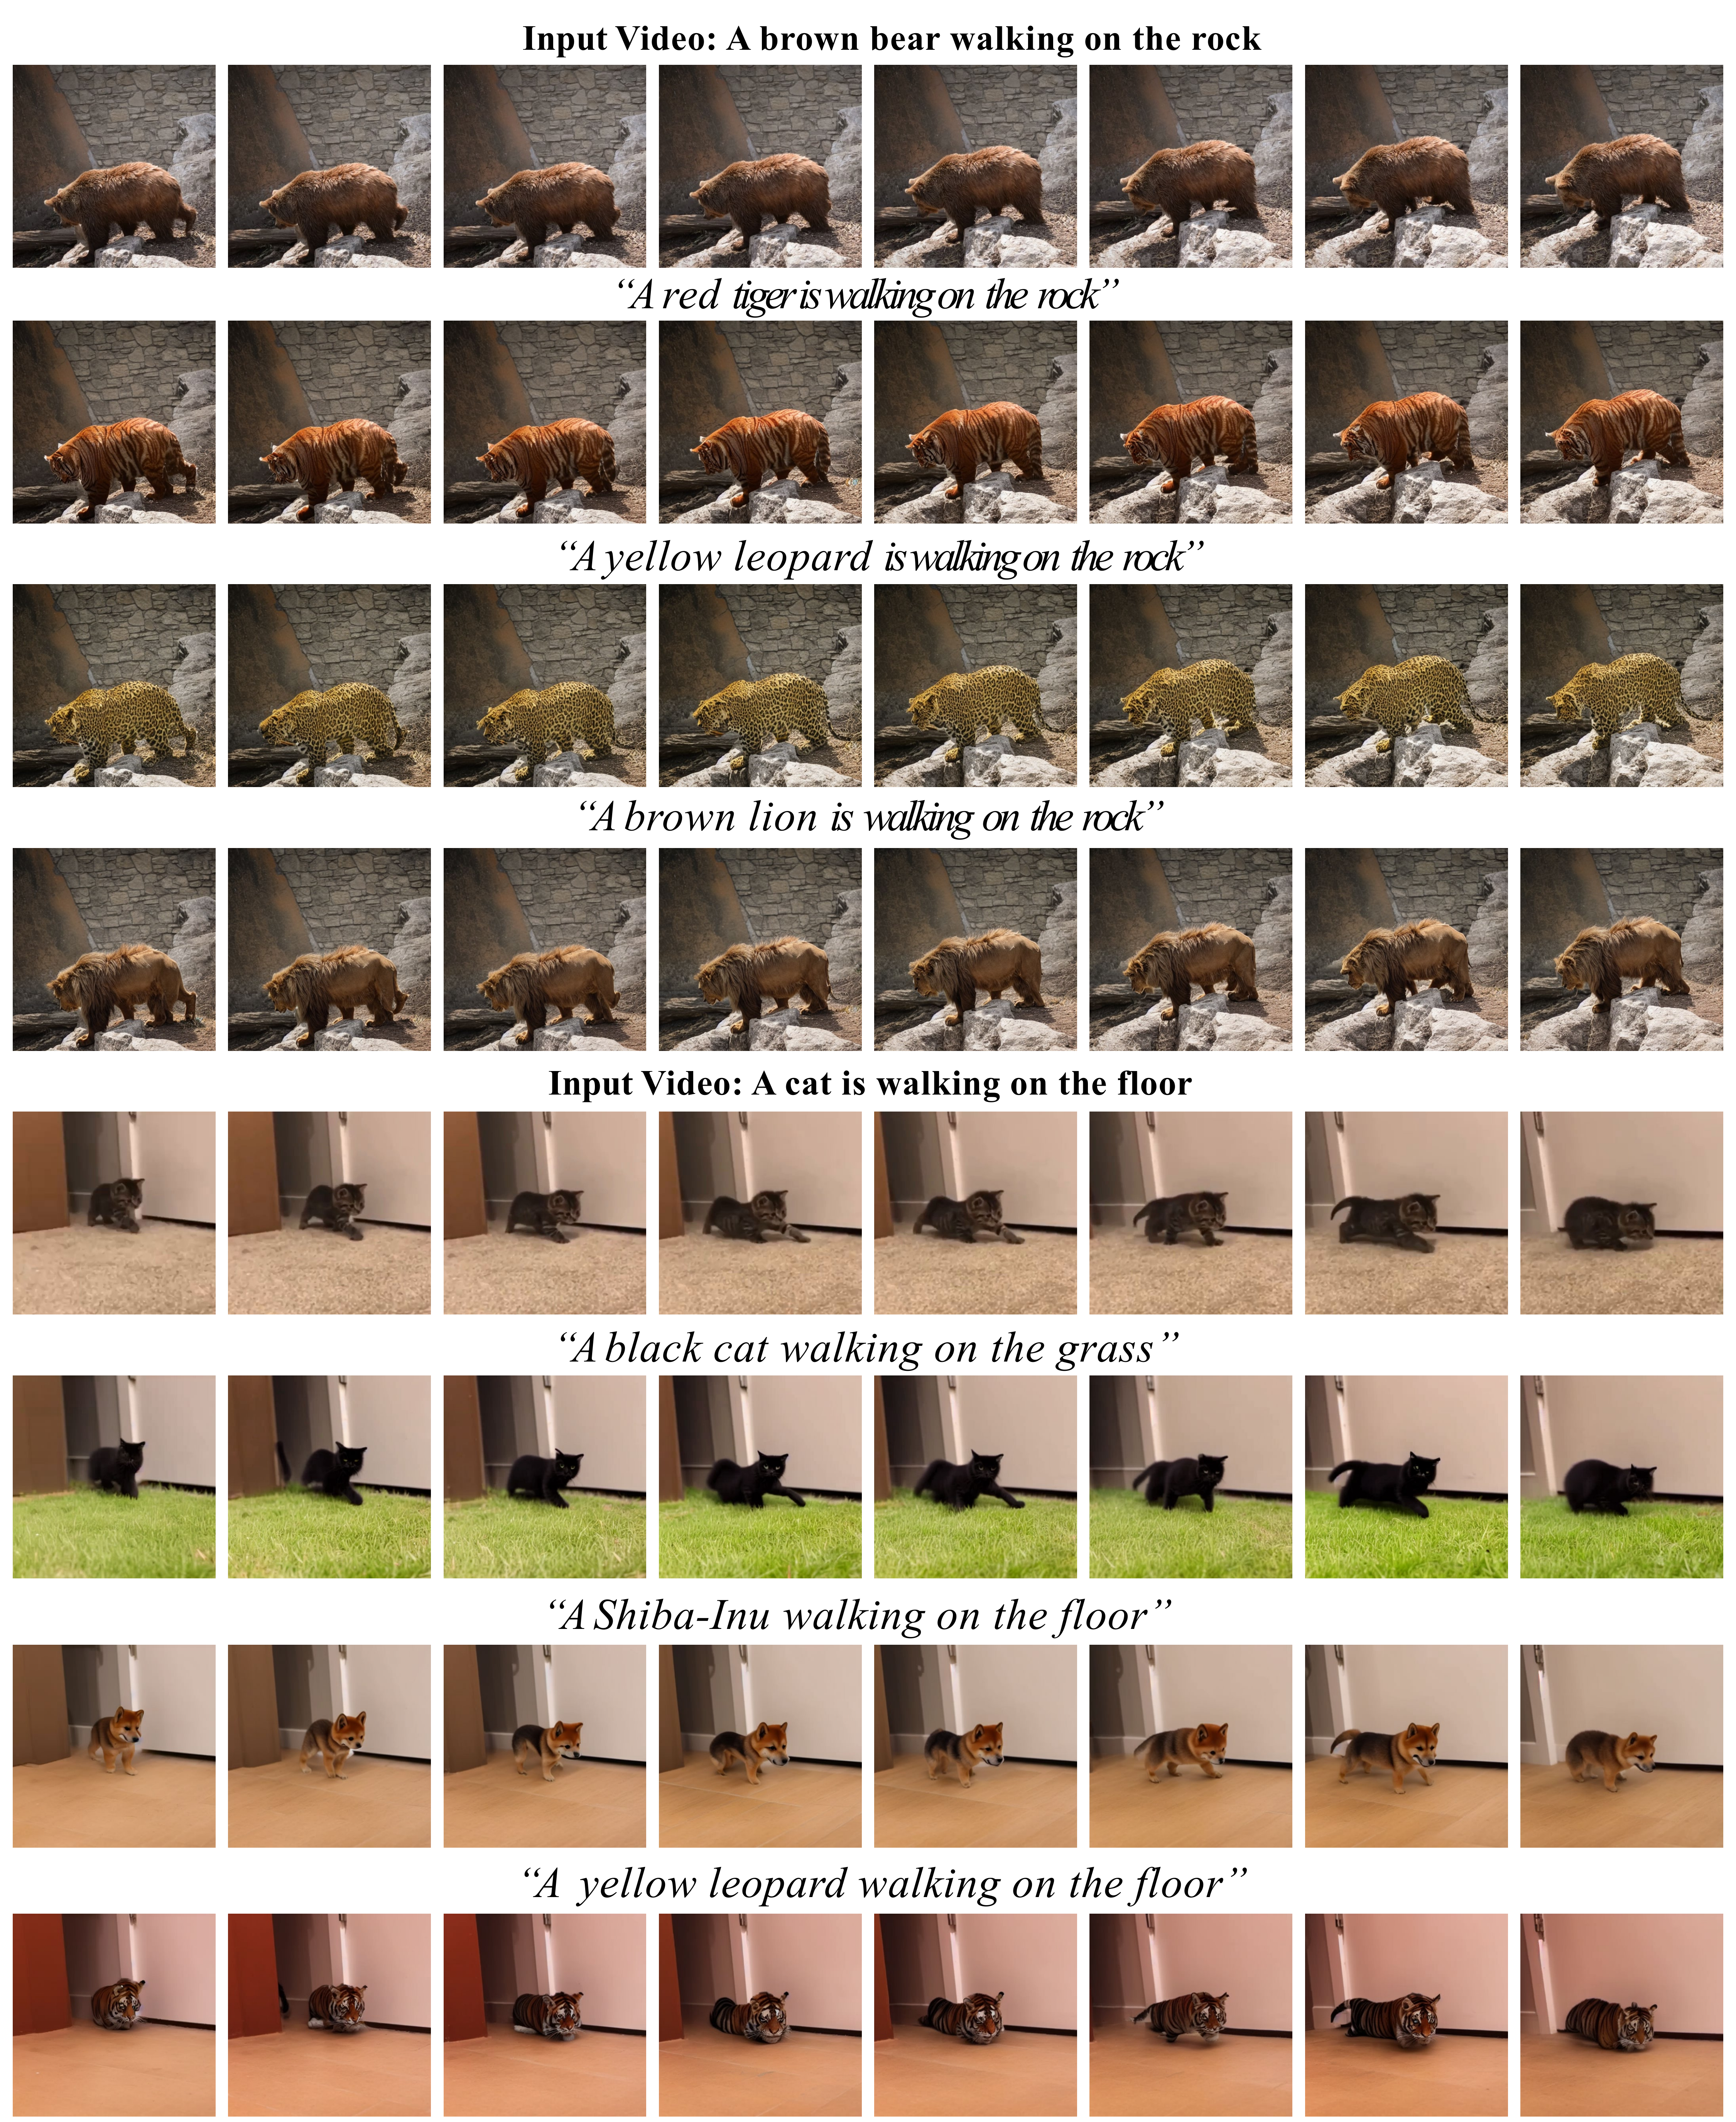}
%    \end{center}
    \caption{\footnotesize{\textbf{Attribute editing with our method}. It can be observed that we have successfully edited the color and animal type in the given input videos. In the first video, the original animal is "bear", which we changed to "red tiger", "yellow leopard", and "brown lion" in the second, third, and fourth rows respectively. Similarly, we changed the original cat's color to black. The results shown in the seventh and eighth rows indicate the ability of our framework to edit according to the animal type and breed in the given prompt. Zoom in for better visibility.} }
\label{fig:leopard}
    
\end{figure*}

\begin{table*}
\caption{\textbf{Quantitative comparison based on User Study}. We compare different T2V generation methods based on user preference. Out of all users, 51.44\% of them prefer \textit{SAVE} when it comes to \textit{frame consistency}.}
\centering
% \resizebox{\columnwidth}{!}{%
\begin{tabular}{lcccc}
\toprule
% {Method} & \multicolumn{2}{c}{CLIP Score}  &  \multirow{2}{*}{Average Editing Time}   \\ \cline{2-3}  
Method &  Frame Consistency & Textual Alignment & Realistic Quality \\ \midrule

CogVideo~\cite{hong2022cogvideo}   & 2.38 &3.25 &4.78\\
Tune-a-Video (TAV)~\cite{wu2022tune}   &7.14&13.09& 13.28\\
Video-P2P\cite{liu2023video} & 39.04      & 38.57  & 38.14  \\  
Ours           & \textbf{51.44} & \textbf{45.09} & \textbf{43.80}   \\ \bottomrule
\end{tabular}%
% }
\label{tab:user}

\end{table*}
\begin{figure*}[t!]
%\begin{center}
\centering
%\hspace{-5mm}
%\begin{minipage}{0.35\textwidth}
    \includegraphics[width=0.7\linewidth, trim={0cm 0cm 0cm 0cm}]{./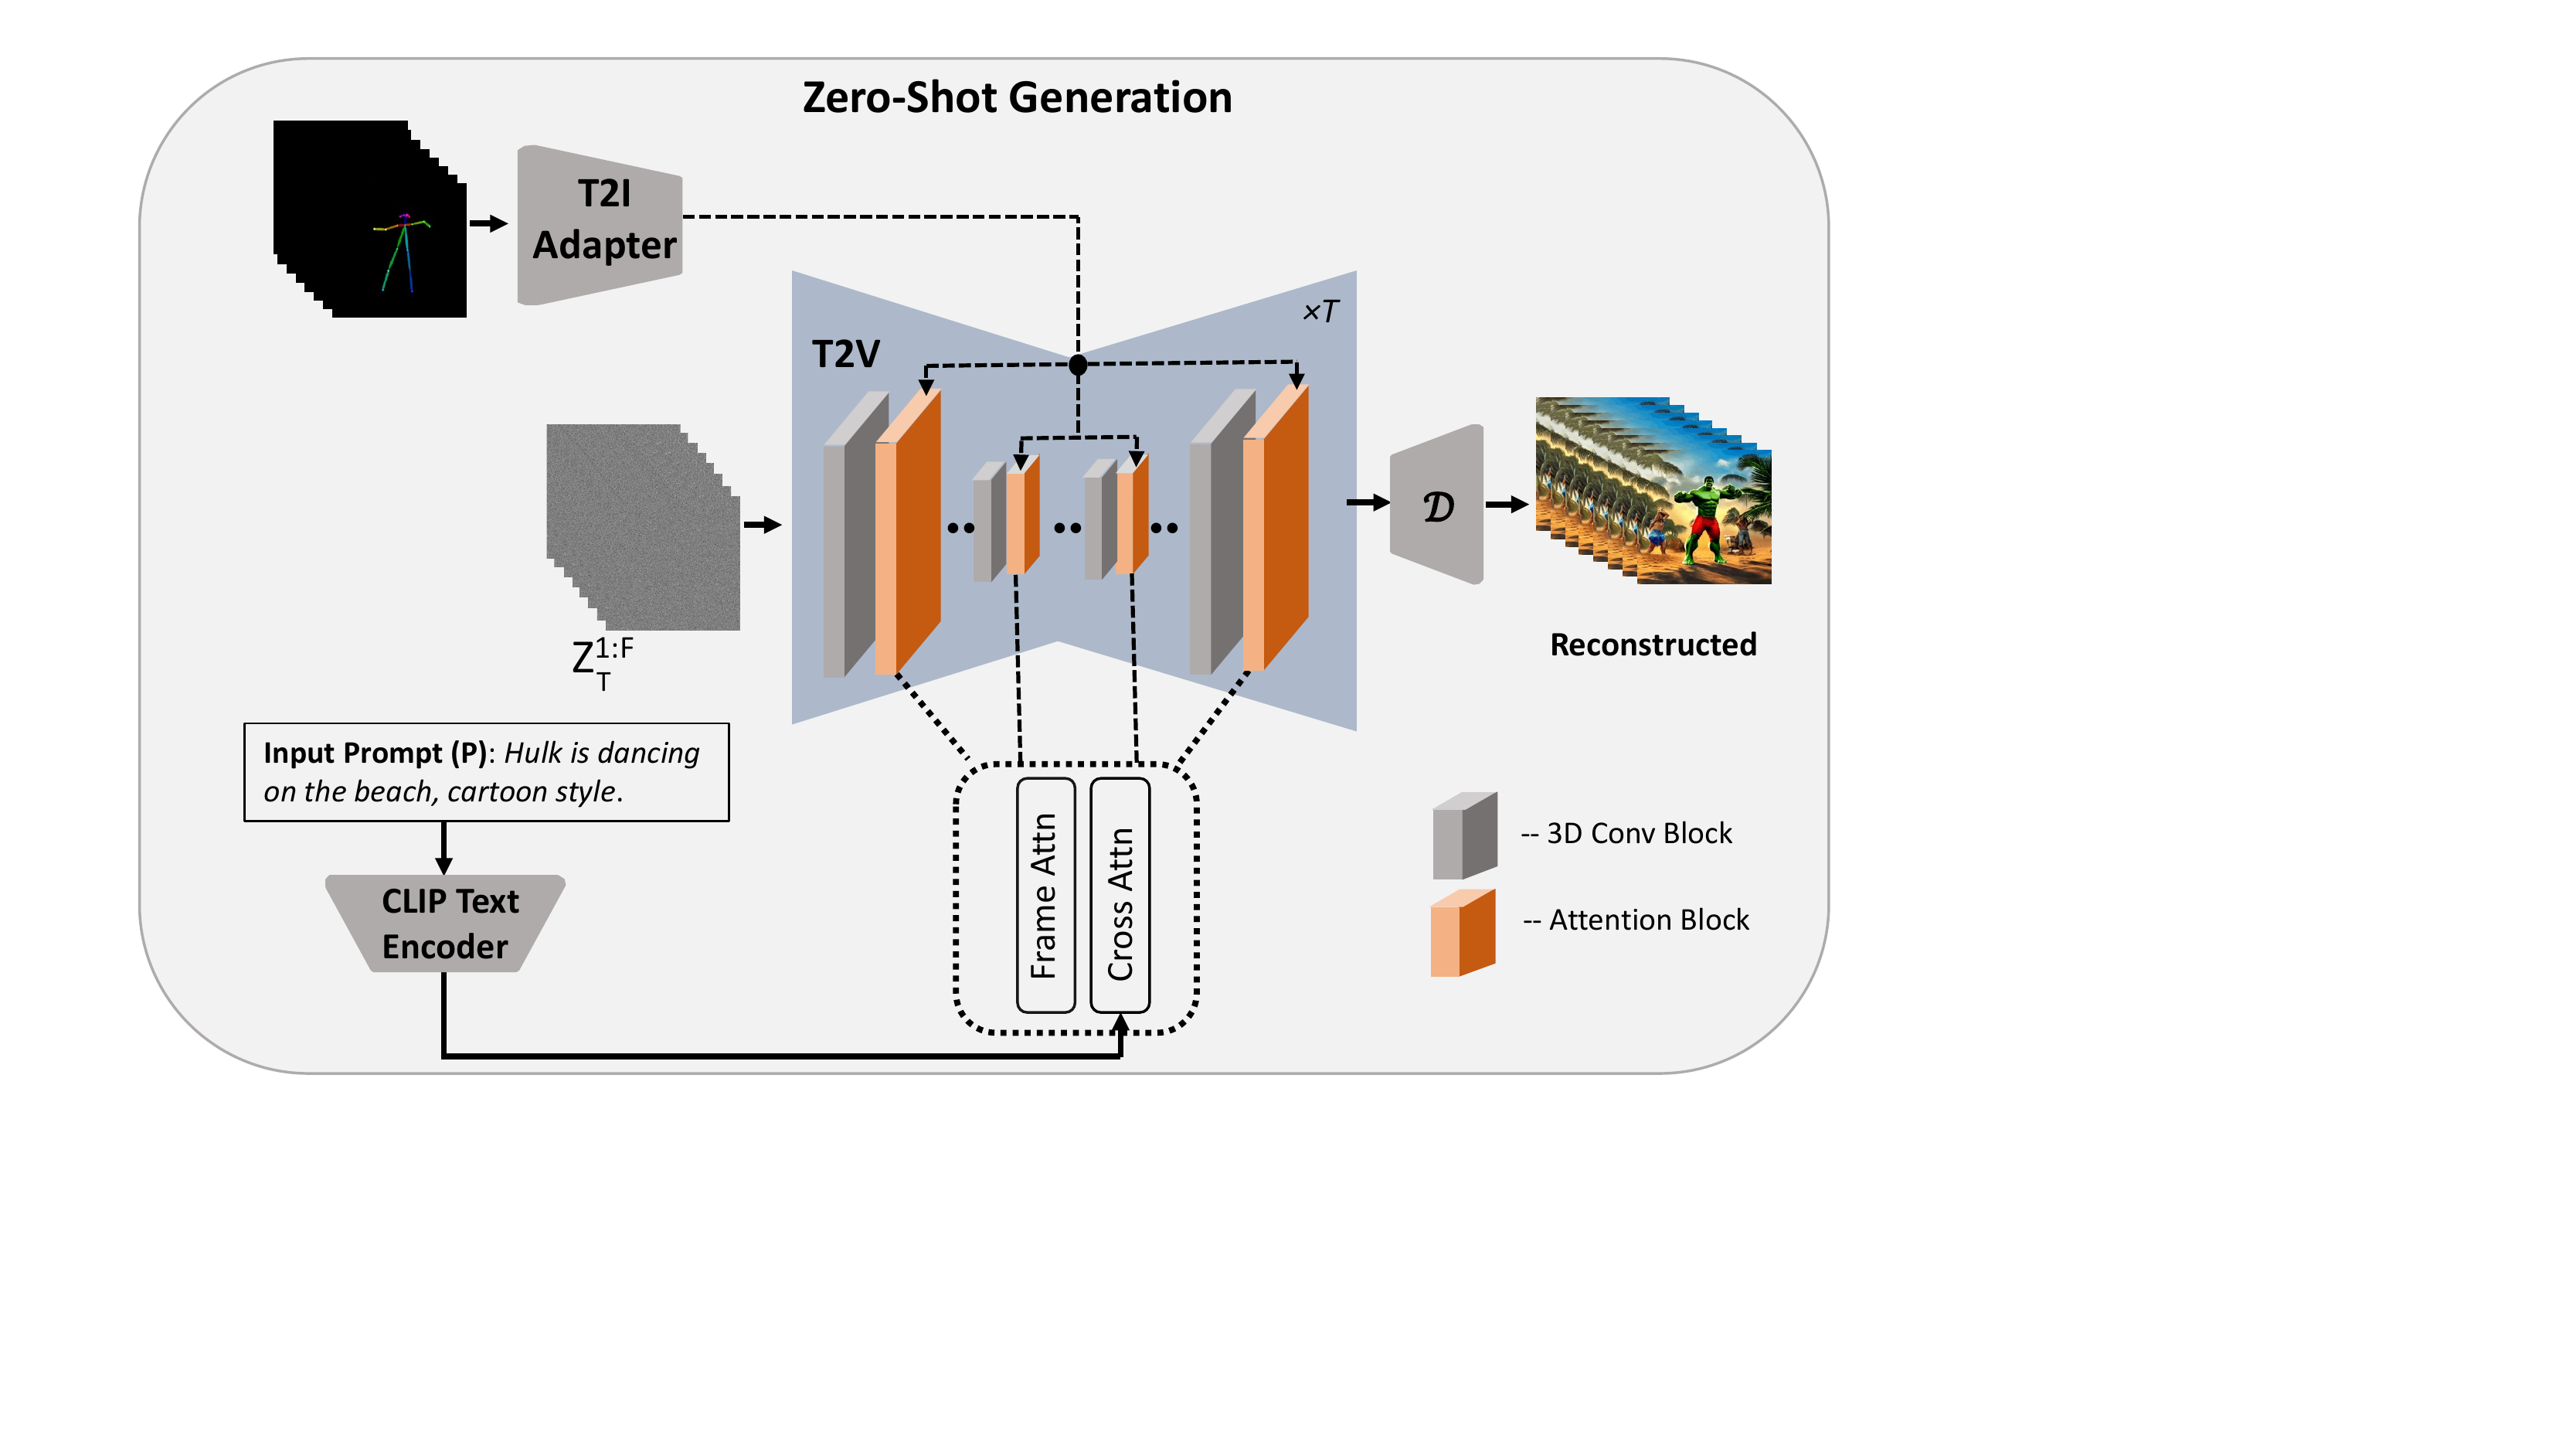}
%    \end{center}
    \caption{\footnotesize{Overview of \textbf{SAVE-Zero-shot text-to-video generation. No training is required} and we do not use any temporal layer. Pre-trained T2I-adapter~\cite{mou2023t2i} is utilized to generate a video with our framework. The T2I adapters capture motion features frame-by-frame with no temporal coherence, which are then integrated with the corresponding frame features of the U-Net encoder blocks. Frame-attention mechanism of the T2V model maintains the temporal consistency within the generated frames of the video.} }
\label{fig:save_zero}
\end{figure*}

\begin{figure*}[htb!] %[t!] %{R}{0.5\linewidth}
%\begin{center}
\centering
%\hspace{-5mm}
%\begin{minipage}{0.35\textwidth}
    \includegraphics[width=0.9\linewidth]{./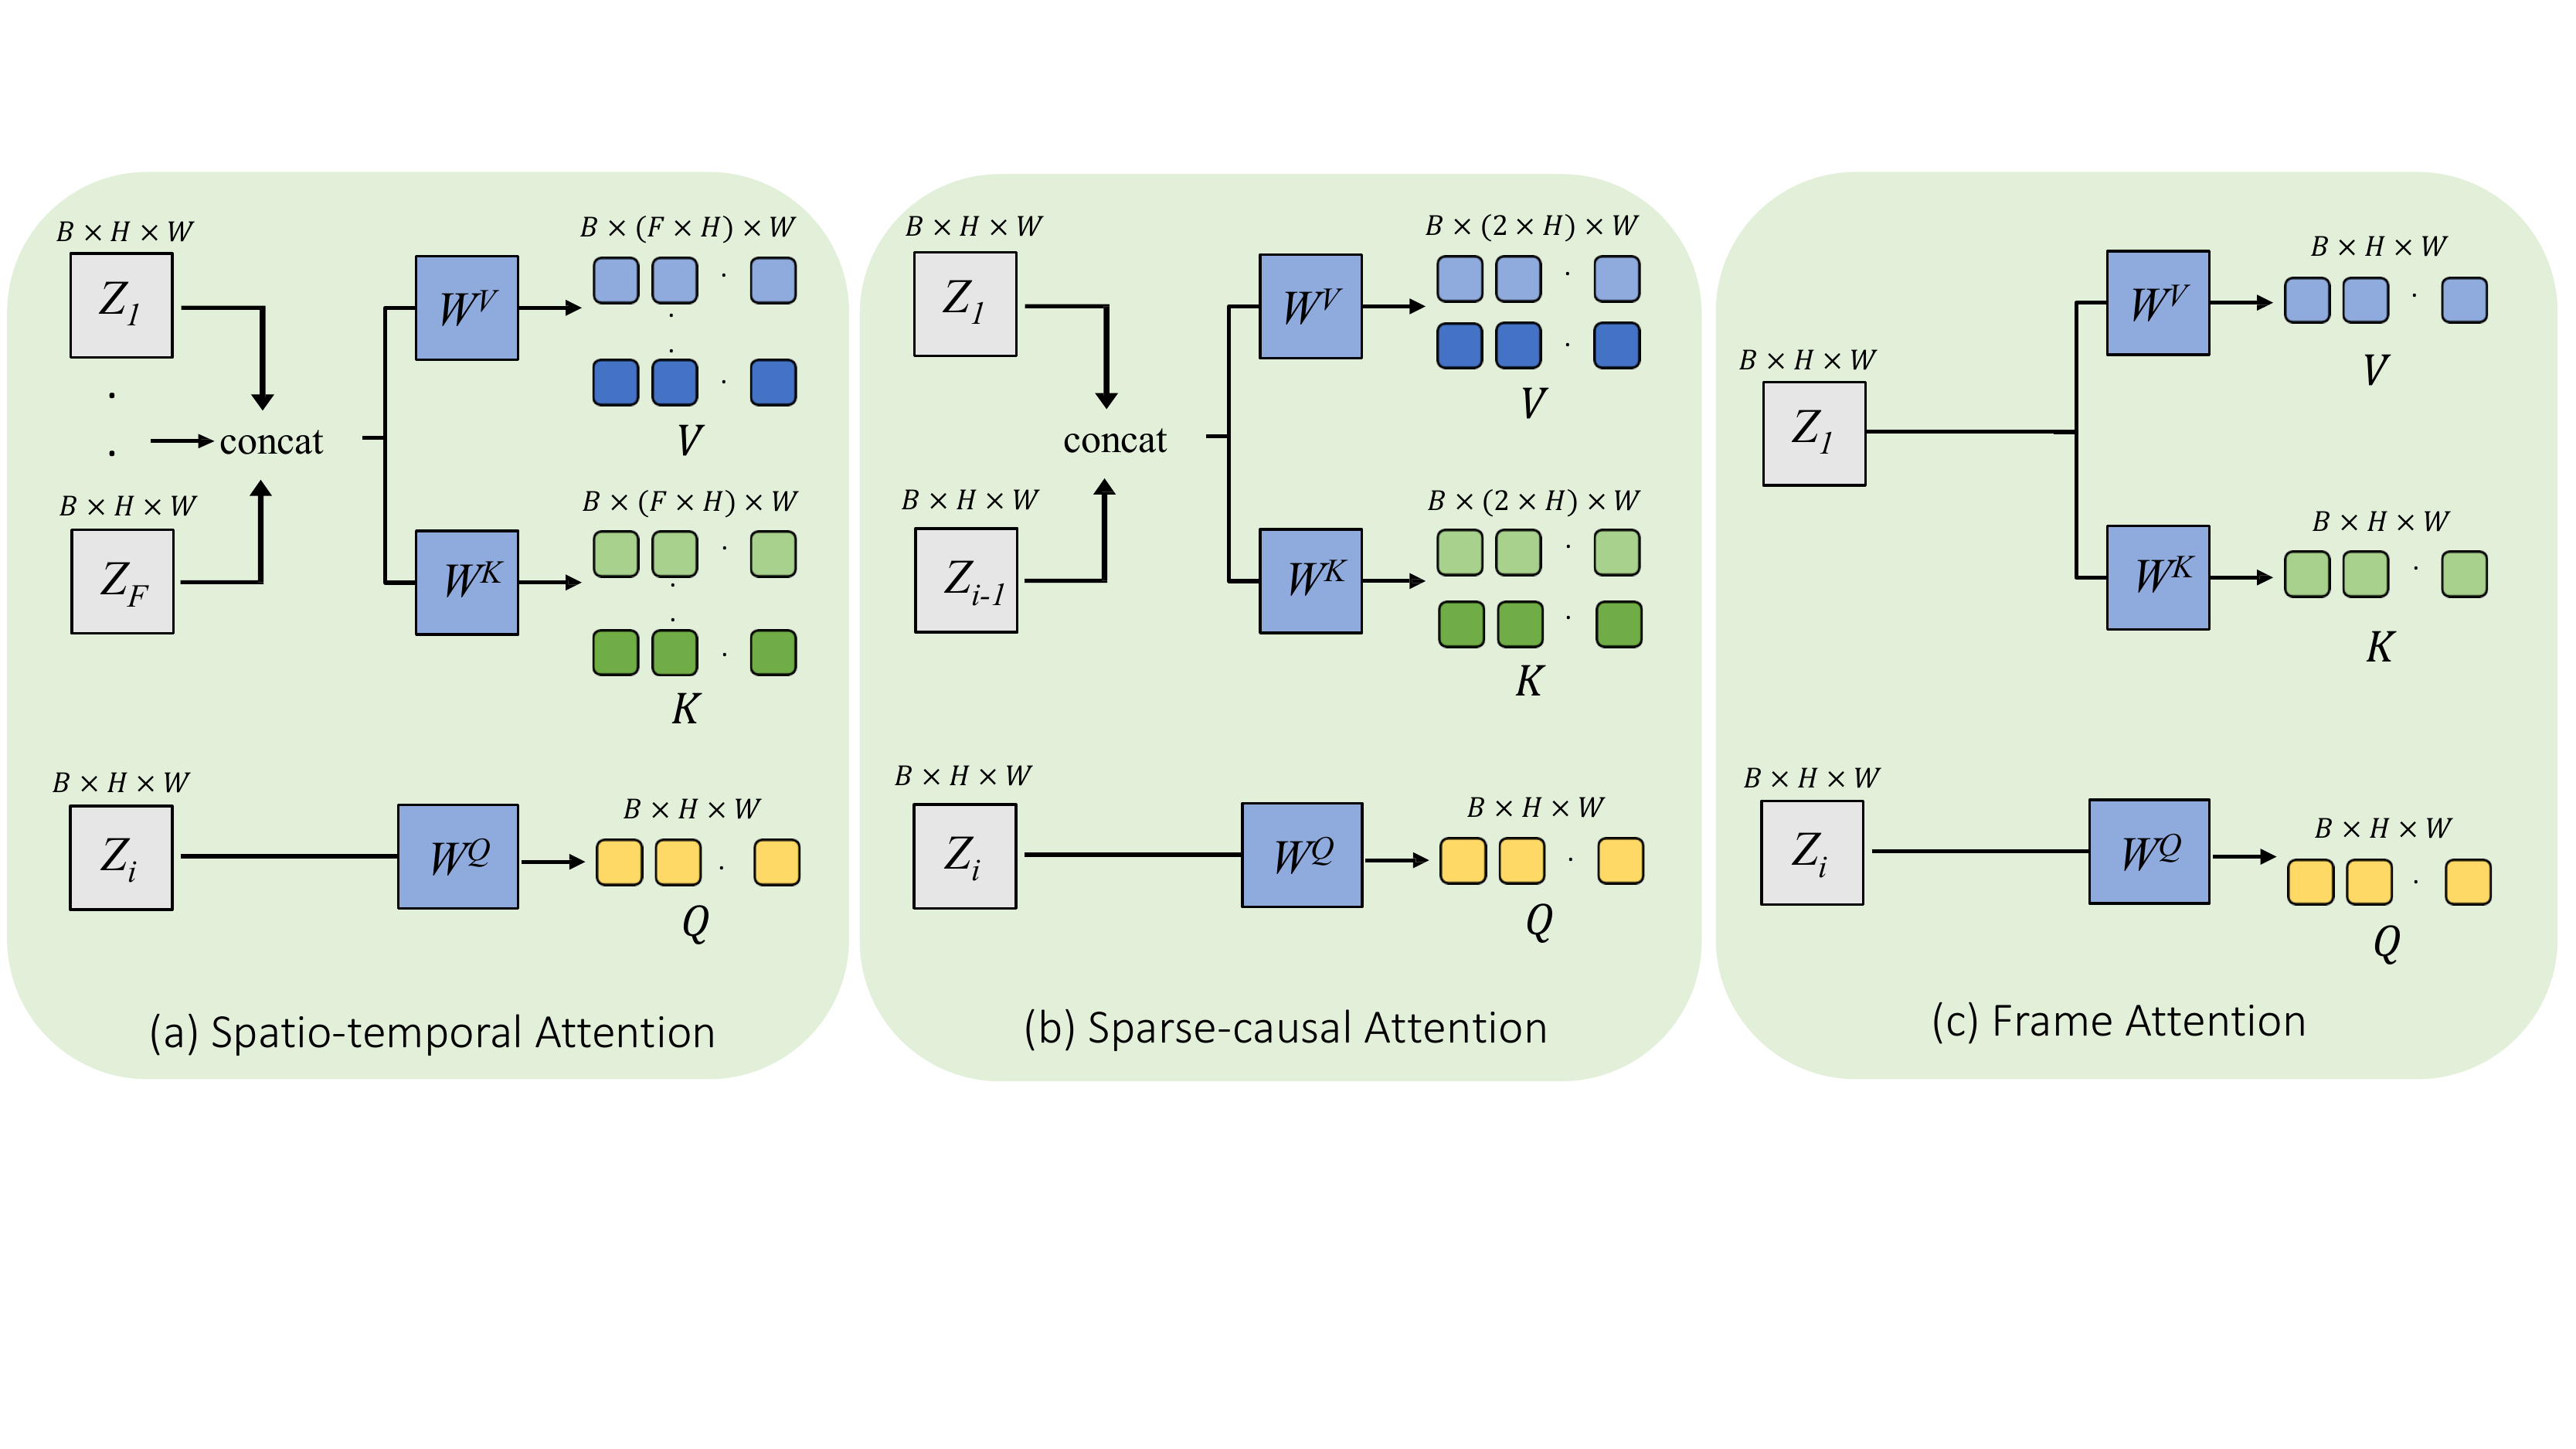}
%    \end{center}
    \caption{\footnotesize Various \textbf{cross-frame attention mechanisms}. We utilize only frame attention in our zero-shot generation approach. Here, no extra parameters are tuned to calculate the attention. We only replace the self-attention with the frame-attention such that the "Key", and "Value" always consist of the first frame latent features. }
\label{fig:attn_cost}
\end{figure*}

\begin{figure*}[t!]
%\begin{center}
\centering
%\hspace{-5mm}
%\begin{minipage}{0.35\textwidth}
    \includegraphics[width=0.9\linewidth]{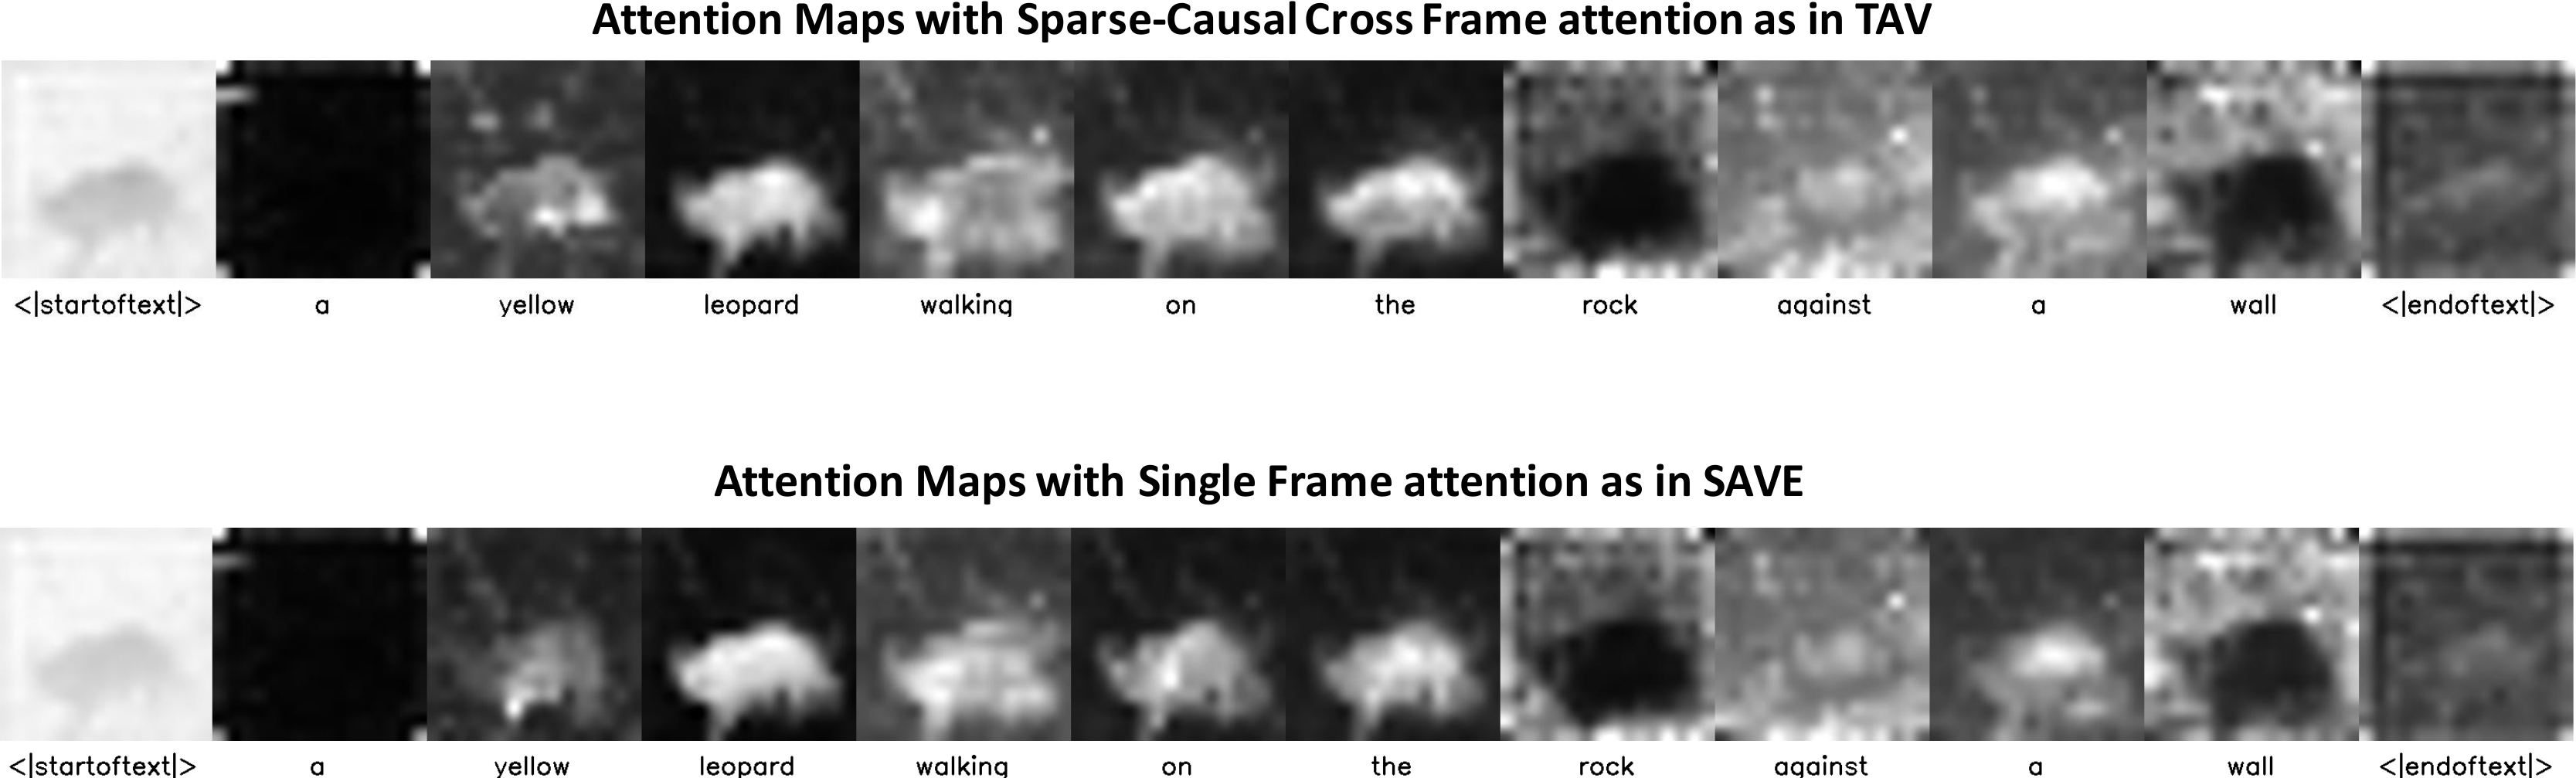}
%    \end{center}
    \caption{\footnotesize{\textbf{Comparison of Sparse-causal and Frame Attention}.Even though both of them perform similarly, frame attention requires significantly less computational resources as compared to Sparse-causal. Zoom in for better visibility. }}
\label{fig:attention_effect}
\end{figure*}

\begin{figure*}[htb!]
%\begin{center}
\centering
%\hspace{-5mm}
%\begin{minipage}{0.35\textwidth}
    \includegraphics[width=1\linewidth, trim={0cm 0cm 0cm 0cm}]{./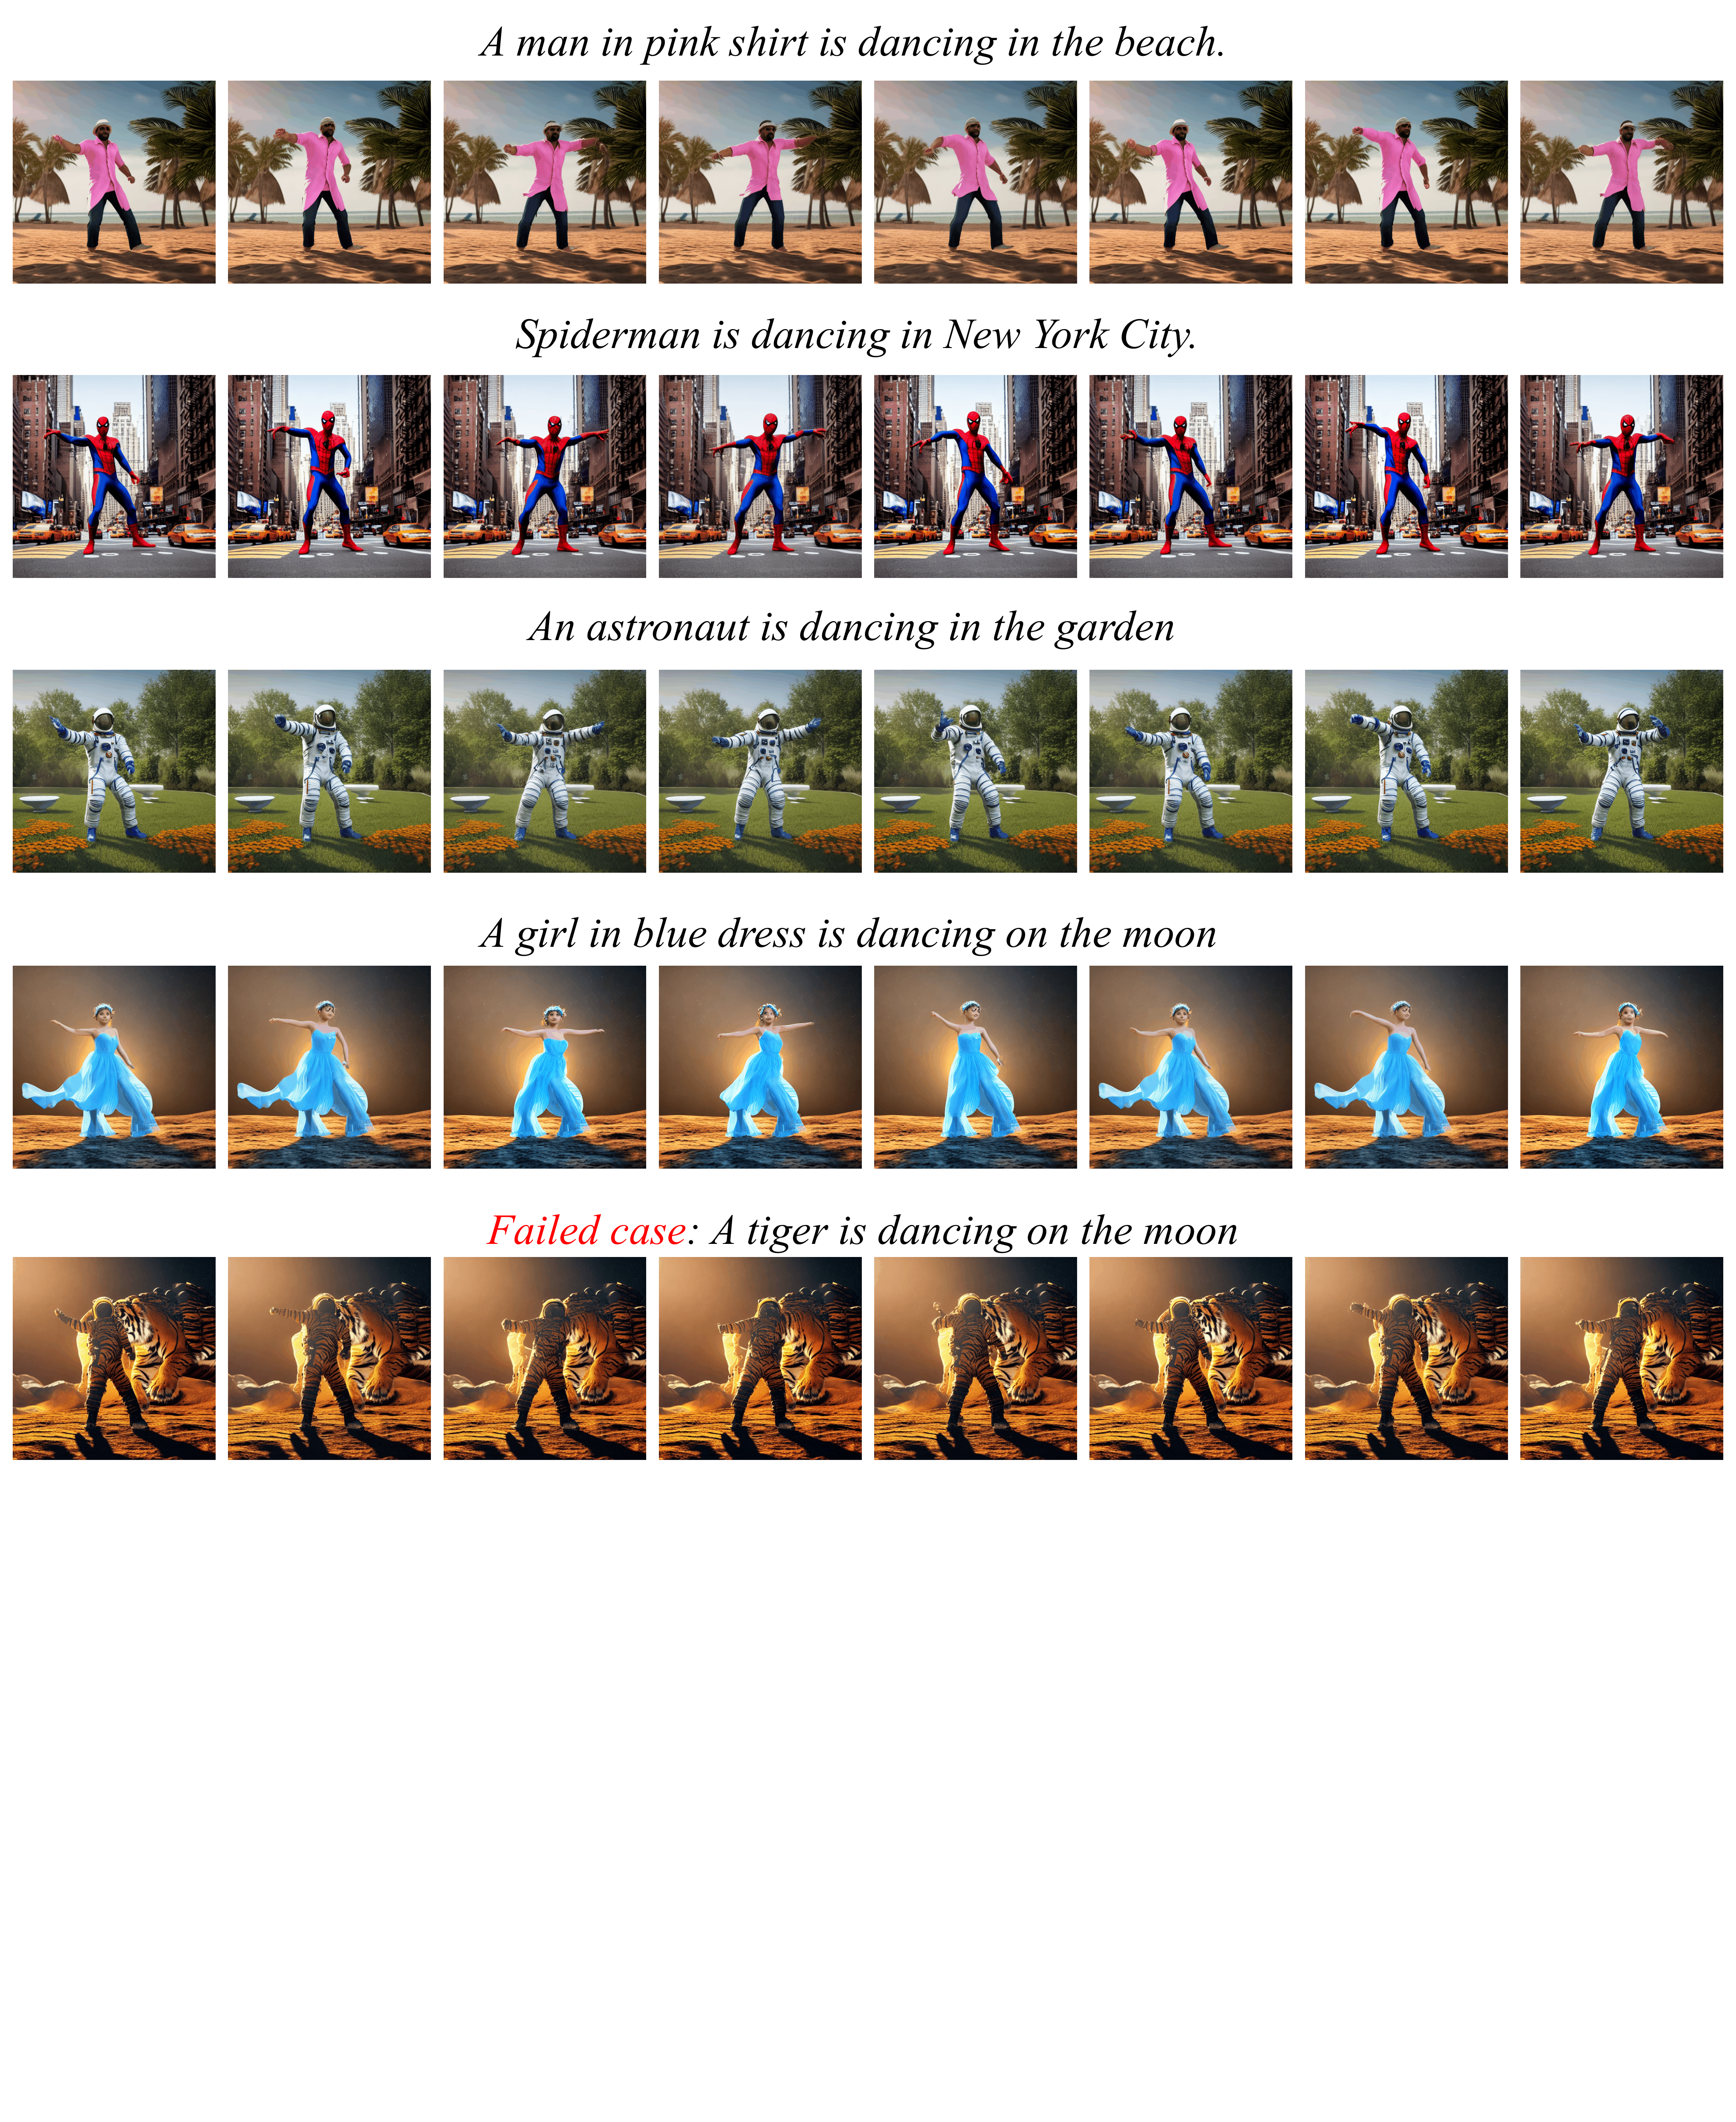}
%    \end{center}
    \caption{\footnotesize{\textbf{Zero-shot video generation with given poses without any training.} We do not use the temporal attention layer in this particular setting. Instead, we use poses and a pre-trained T2I adapter to inject the motion information into the generation process. A \textit{failure case} has also been shown here where the model is struggling to replace the human subject with an animal, e.g. tiger, bear, etc. In this case, the motion information is not fully transferable as the tiger cannot move/dance like a human. Although the model generates a tiger-like object due to hard-to-transfer motion information the model also keeps the human subject. Zoom in for better visibility.}}
\label{fig:vid_zero_pose}
\end{figure*} 
\begin{figure*}[h!]
%\begin{center}
\centering
%\hspace{-5mm}
%\begin{minipage}{0.35\textwidth}
    \includegraphics[width=1\linewidth, trim={0cm 0cm 0cm 0cm}]{./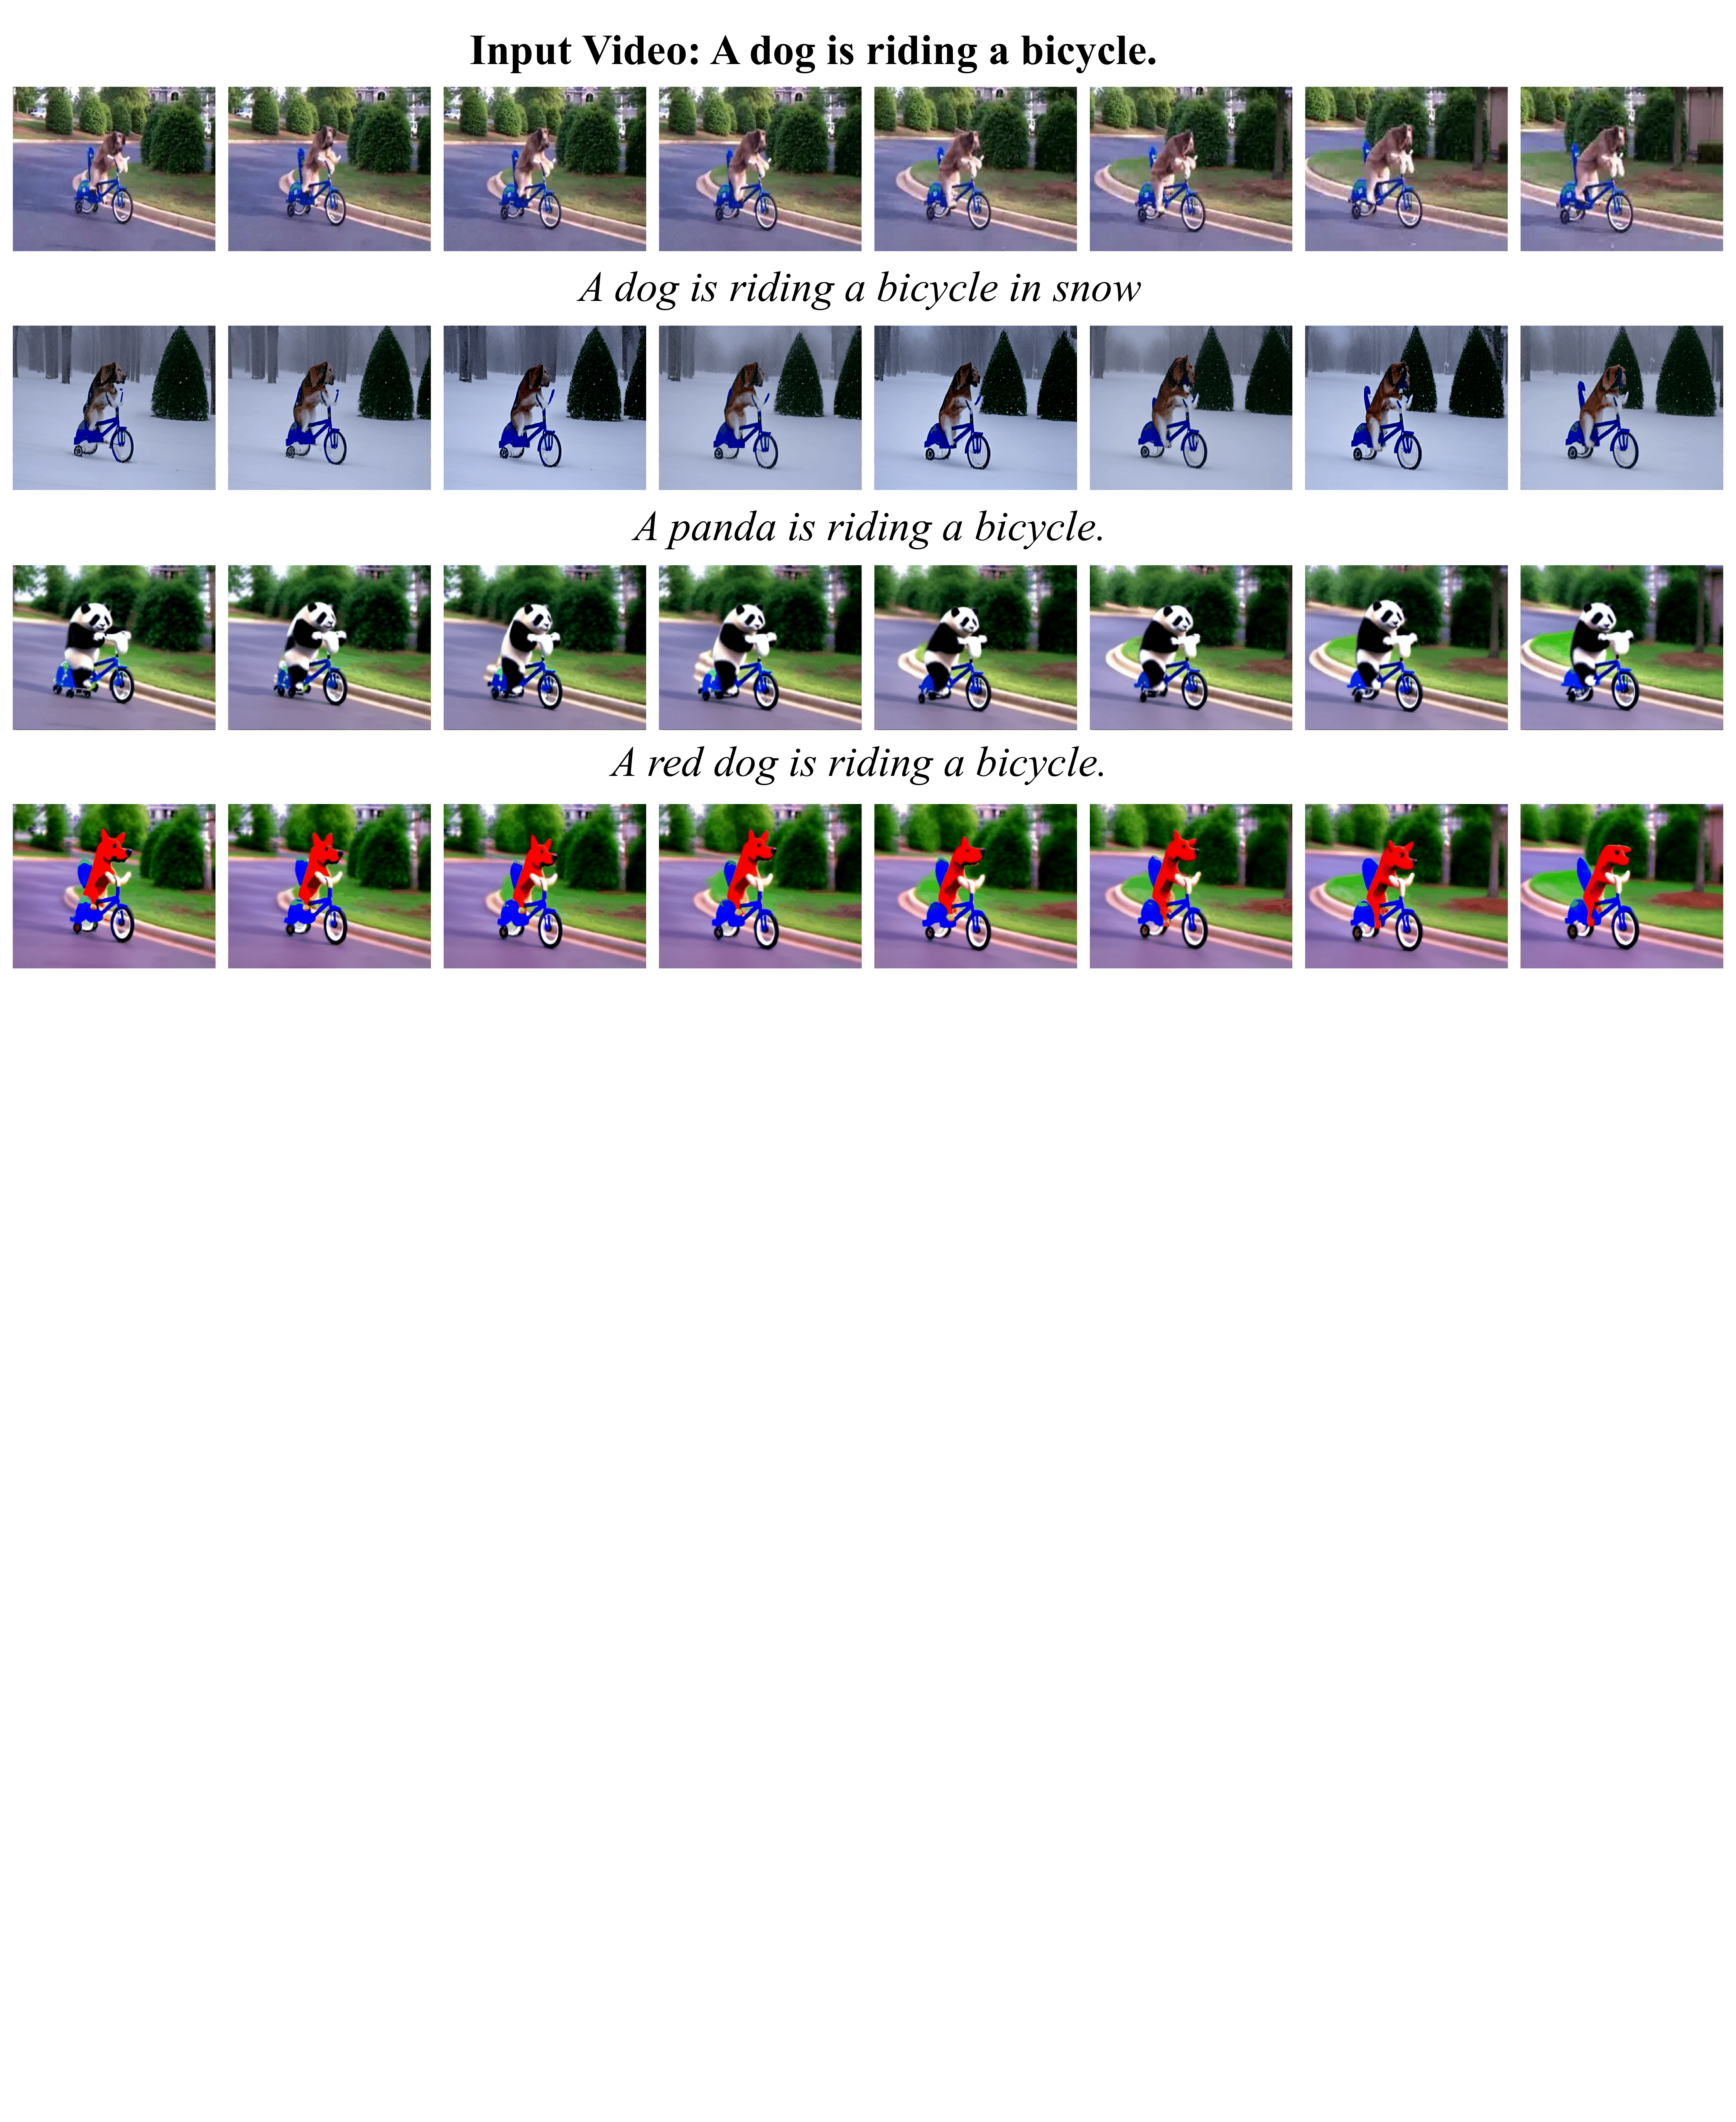}
%    \end{center}
    \caption{\footnotesize{\textbf{Video editing results} on diverse input video using SAVE framework.} }
\label{fig:dog_only}
    
\end{figure*}
\begin{figure*}[h!]
%\begin{center}
\centering
%\hspace{-5mm}
%\begin{minipage}{0.35\textwidth}
    \includegraphics[width=1\linewidth, trim={0cm 0cm 0cm 0cm}]{./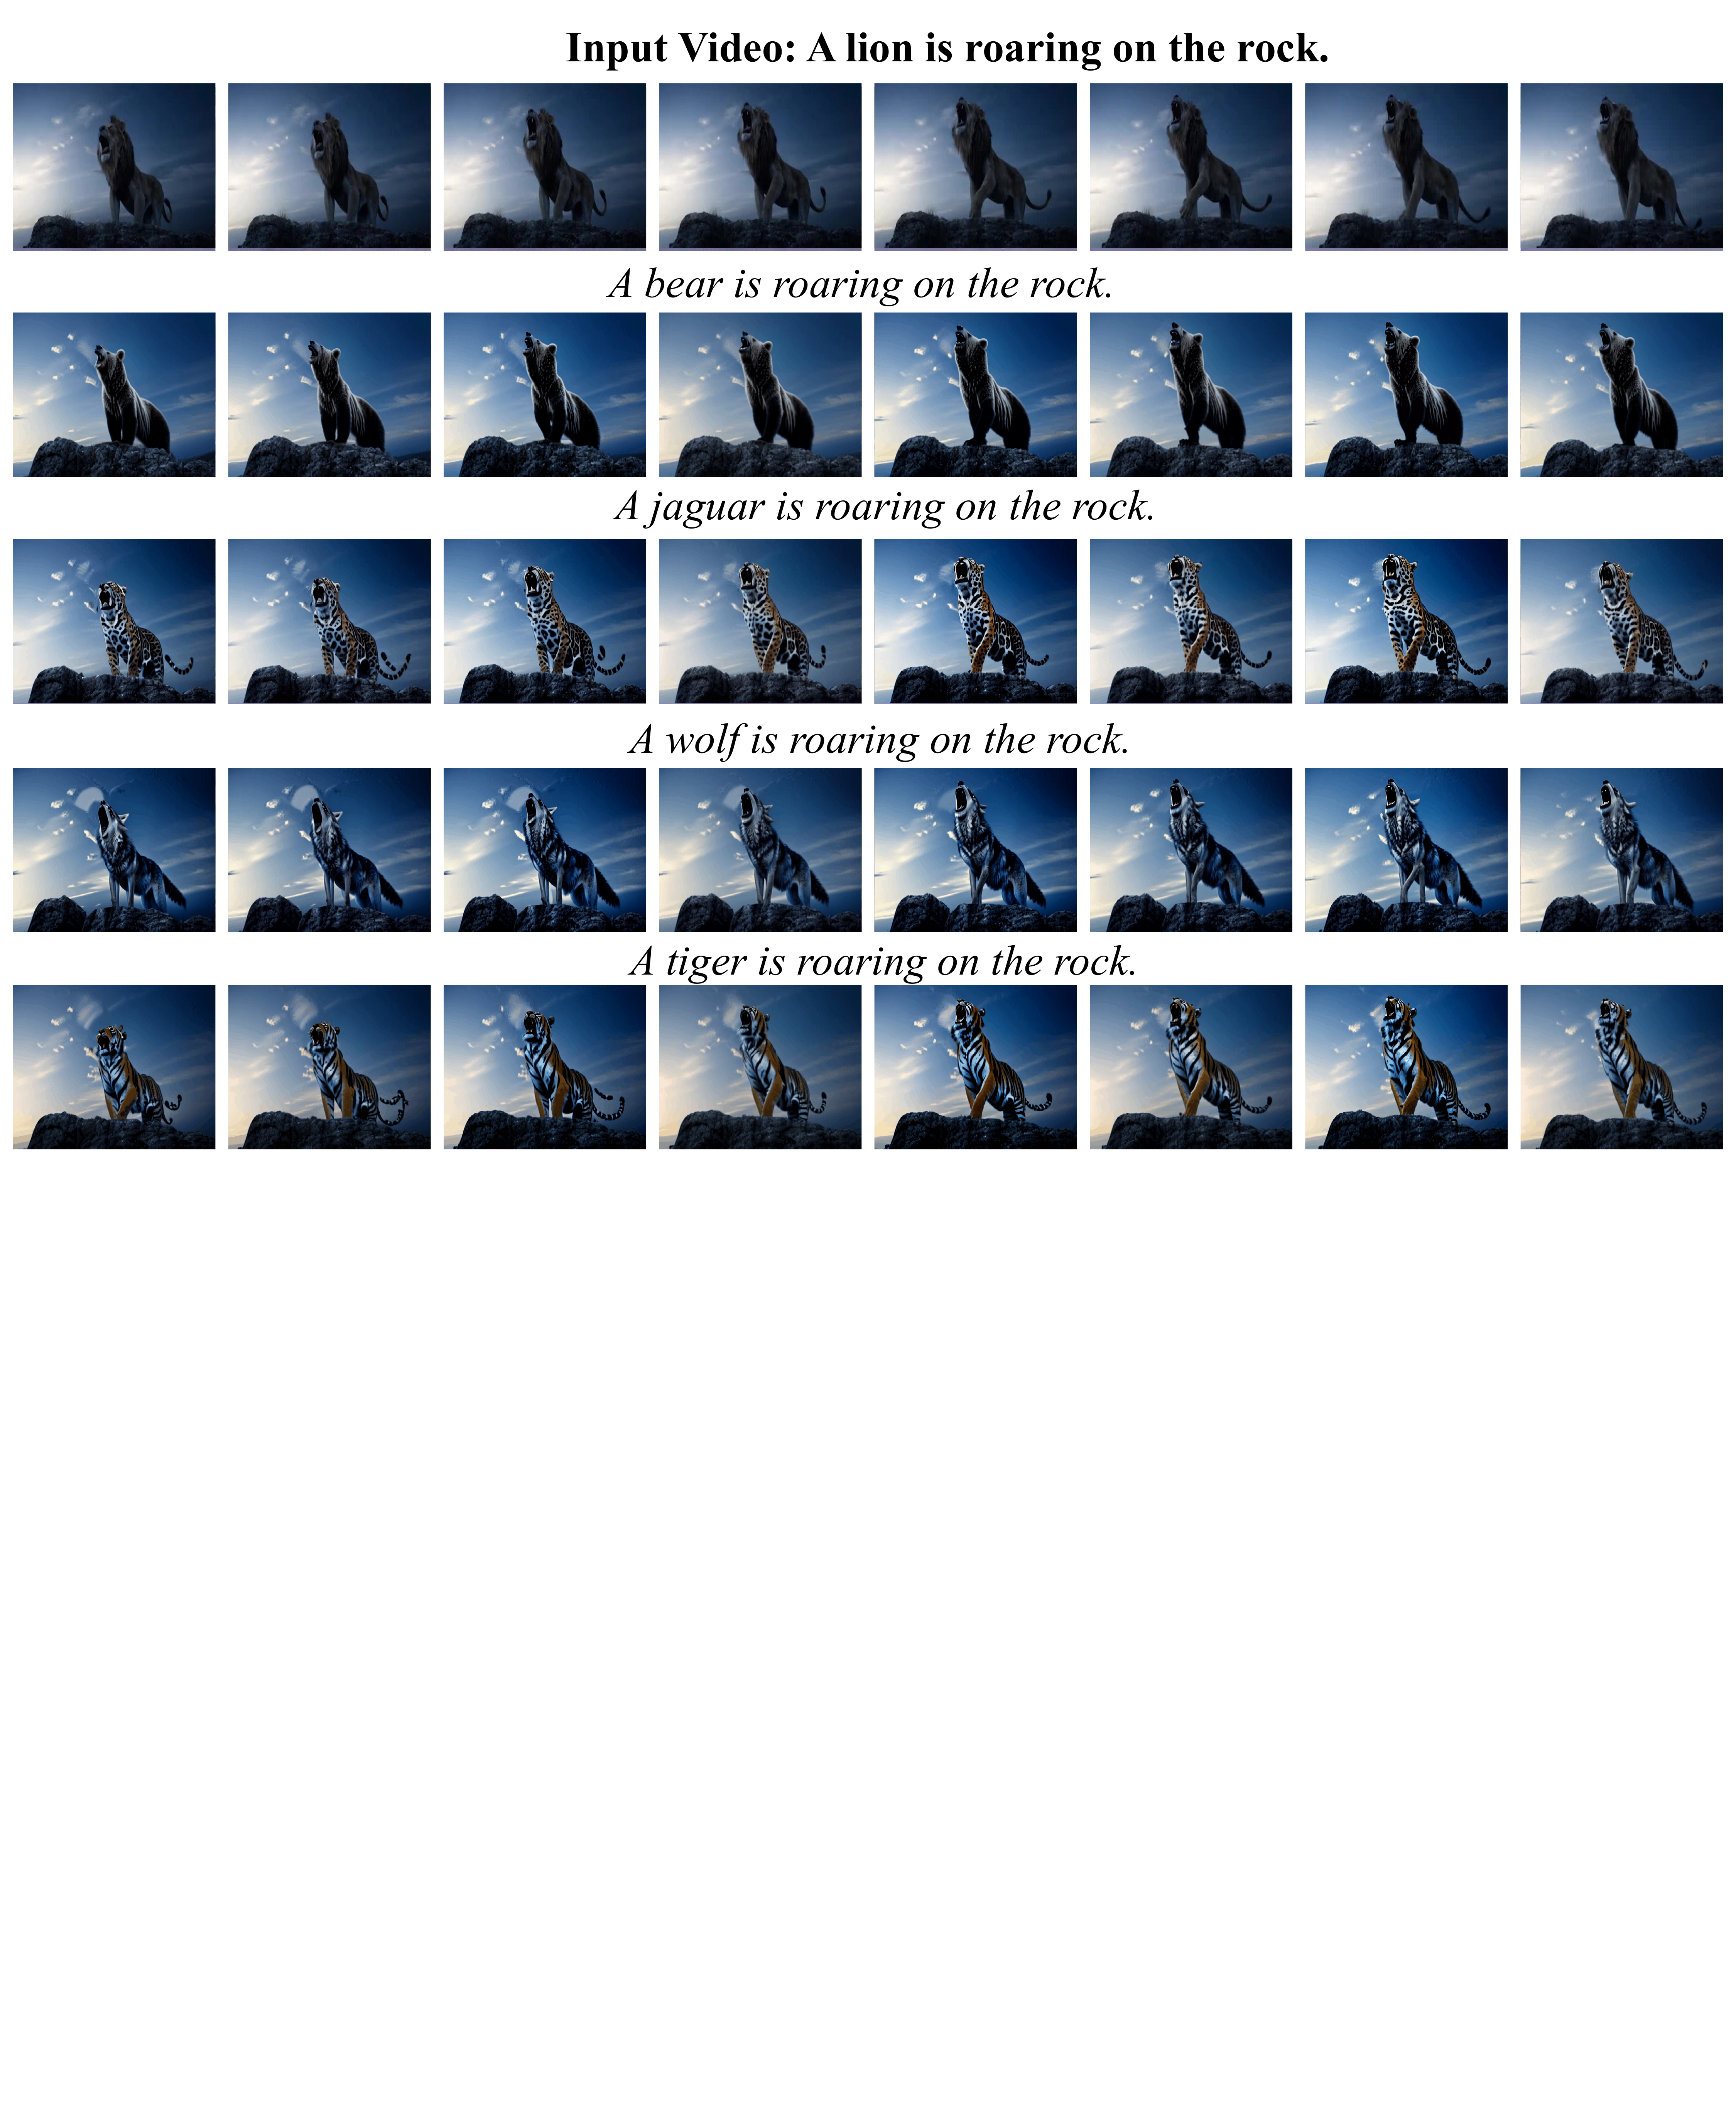}
%    \end{center}
    \caption{\footnotesize{\textbf{More video editing results} using SAVE framework where a lion is replaced with other animals using the editing text prompt. Zoom in for better visibility.} }
\label{fig:lion}
    
\end{figure*}
\begin{figure*}[htb!]
%\begin{center}
\centering
%\hspace{-5mm}
%\begin{minipage}{0.35\textwidth}
    \includegraphics[width=1\linewidth, trim={0cm 0cm 0cm 0cm}]{./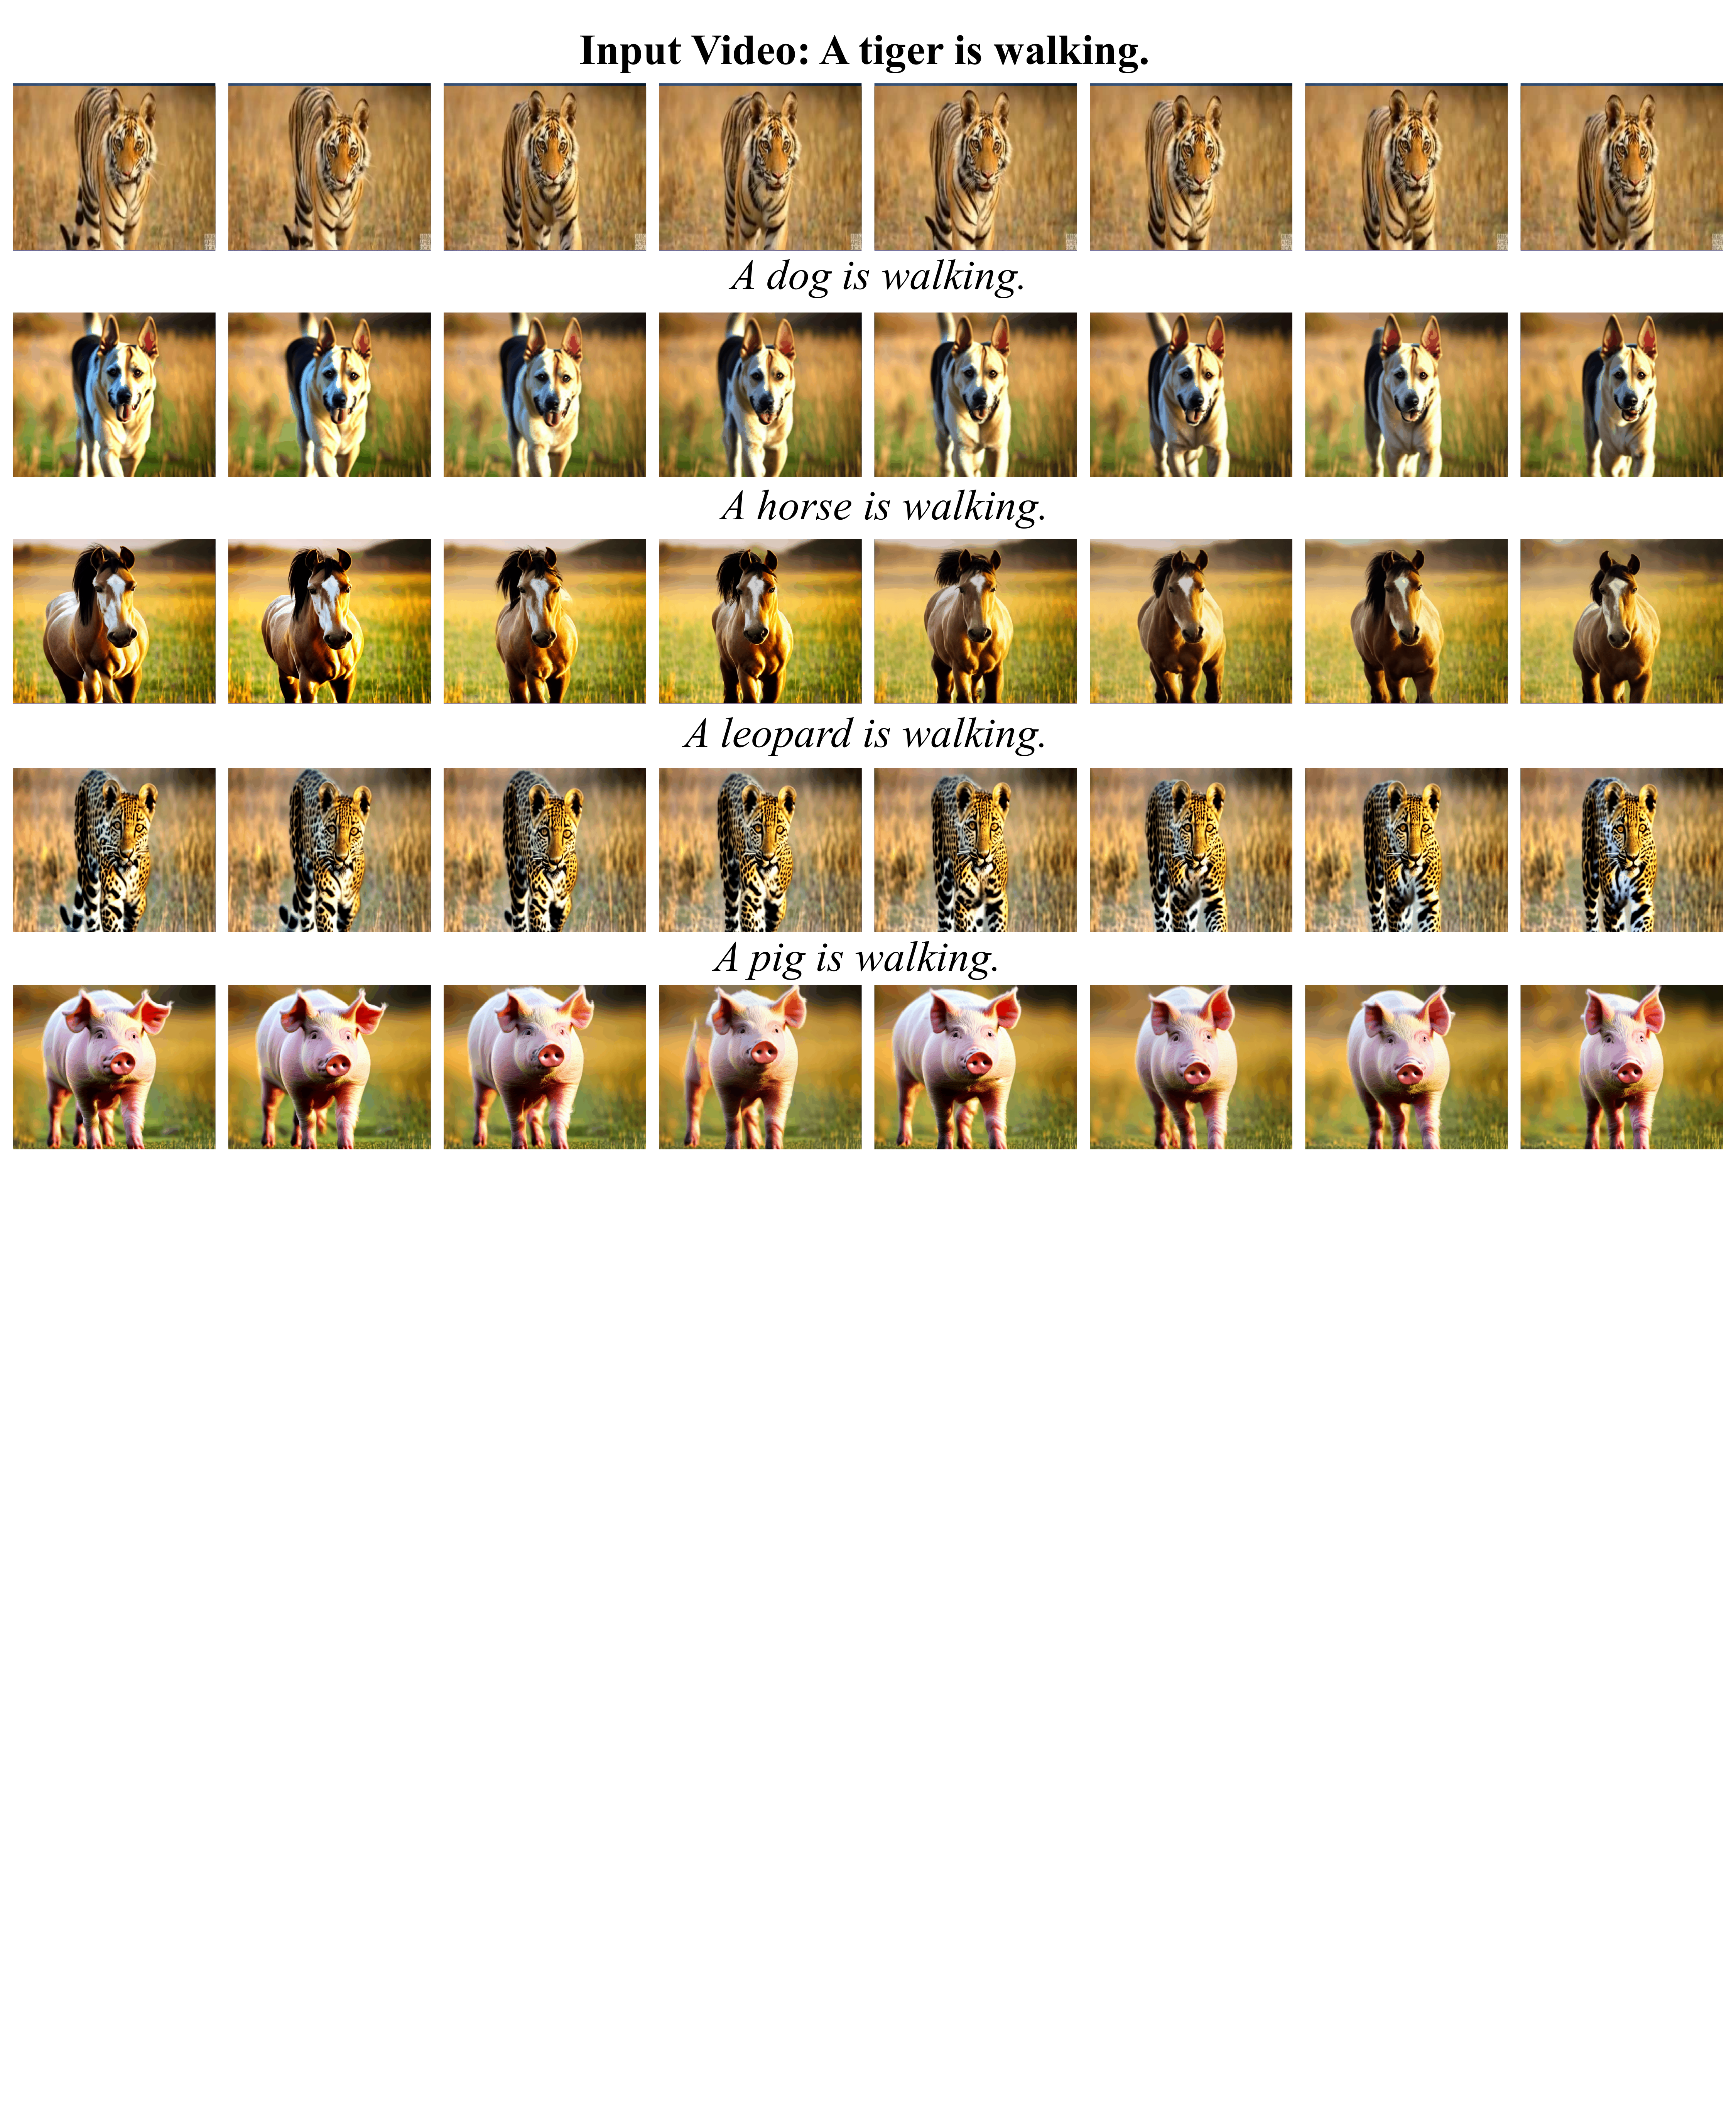}
%    \end{center}
    \caption{\footnotesize{\textbf{Video editing results} using SAVE framework where a tiger is replaced with other animals using editing prompts. Zoom in for better visibility.} }
\label{fig:tiger}
\end{figure*}

\section{More on Spectral Shift Optimization}\label{sec:motivation}
Figure~\ref{fig:lgn} shows how regularization of spectral components is able to generate more diverse and statistically similar samples to the original samples. There are three sets of generated samples using 400 samples of AT\&T face dataset \cite{samaria1994parameterisation}. In the first row, the mean and variance of each pixel are used to generate a new random sample. In the second row, a new random sample is generated by a random and unconstrained combination of spectral components. While the third row shows pursuing singular values of the original dataset results in more naturally generated samples.  Figure \ref{fig:att_svs} shows the spectrum of the original dataset and the generated samples using a regularized combination of singular vectors.  Adapting the spectral coefficients change the generation capability leading to different outputs. In the case of DNN based generator, the weights control the generation capability. Adapting the spectral shift of weights operates similarly to adapting the spectral coefficients of a linear generator. Although DNN is a more powerful generator and requires more care while adapting.

\subsection{Coarse vs Fine-Matching}
In our work, we proposed a spectral shift regularizer for fine-grained control of the overall editing. We use terminology such as coarse-matching and fine-matching to better describe the reflection of textual command on the edited contents in the video. In summary, these terms describe whether the edited video accurately reflects the
target text condition. The "coarse matching" involves the initial alignment or broad association of textual descriptions with features present in the diffusion-edited image. This phase aims to establish a general correspondence between the provided text and the visual elements within the image. In contrast, "fine-matching" delves into a more detailed and precise alignment between the specific elements mentioned in the text description and the nuanced details or finer aspects within the diffusion-edited image. It focuses on pinpointing and aligning intricate details or specific features referenced in the text with corresponding visual elements present in the image. 

Figure~\ref{fig:effect_regularizer} shows the model attention maps with and without the regularizer. Our goal is to keep the special token's attention from being spread out any further than the coarse class token. The proposed regularizer is able to achieve that by producing more compact cross-attention maps. We also show additional examples of such compactness in Figure~\ref{fig:additiona_eefect_regular}. Further analysis shows the impact of this on the local editing and multi-object as well. (\textcolor{magenta}{Please see the attached PPT})  

% In Figure~\ref{fig:confusion_matrix}, we present the correlations of spectral shifts that are learned individually from different videos. For each non-diagonal entry, we take the average cosine similarity, \textit{Cos-Sim}, between the spectral shifts of two videos. We take this average across all layers. The diagonal entries show the correlation of spectral shifts for two learning rates and the same video. The results indicate that spectral shift learned under different training settings is capable of capturing the underlying concept in the video. Furthermore, conceptually similar videos have high cosine similarity.    

\section{SAVE Algorithm}\label{algo}
We present the algorithm of our proposed video editing framework in Algorithm~\ref{alg:attention}.\\

\section{Additional Results}\label{additional_results}
% \textcolor{cyan}{UMAR, can we generate results for more dataset. I can also help. This will increase our chances of getting accepted.}
We further present the video editing results from our method in Fig.~\ref{fig:swan_1} and Fig.~\ref{fig:leopard}. The shape editing performance of our method can be observed in Fig.~\ref{fig:swan_1} where a swan is replaced with a duck, pelican, and flamingo. Further, the attribute editing results have been illustrated in Fig.~\ref{fig:leopard}, where editing is performed with a specific color or dog breed. More editing results can be observed in Figures ~\ref{fig:dog_only}-~\ref{fig:tiger}.

\section{User Study Details}\label{userstudy}
We conducted a user study to assess \textit{frame consistency}, \textit{textual alignment}, and \textit{realistic quality}. The study involved presenting four videos generated by our method, as well as baselines, to raters in a randomized order. The raters were tasked with evaluating temporal consistency for frame consistency assessment and determining video alignment with the given textual description for textual alignment evaluation. Each example was annotated by 20 participants, and the final outcome was determined through a majority vote. This user study allowed us to gather subjective judgments from multiple perspectives and obtain valuable insights into the perceived quality and alignment of the generated videos with respect to frame consistency and textual faithfulness. The results are shown in Table~\ref{tab:user} 

% We conduct a user study on our dataset of 140 edited prompts to compare our method against two baselines: Plug-andPlay [44] and CogVideo [19]. The comparison results are shown in Tab. 1. The participants of the user study are mainly
% students and colleagues in university. We ask 5 raters to evaluate each edited prompt by comparing two videos generated by
% two different methods (shown in random order) and answering two following questions:
% 1. Which video has higher consistency? Please select the one that looks more smooth as a video.
% 2. Which video matches the text better? Please select the one that better represents the given text description.

\section{Zero-Shot Text-to-Video Generation}\label{zero-shot} 
We further present \textbf{SAVE-Zero-Shot}, a zero-shot video generator variant of our efficient video editor as shown in Fig.~\ref{fig:save_zero}. Specifically, we aim to produce a video $\mathcal{X}=\{x_i|i\in[1,F]\}$ with $F$ frames for a given prompt $\mathcal{P}$ conditioned on motion sequences $\mathcal{M}=\{m_i|i\in[1,F]\}$ without any fine-tuning. To achieve this, we propose a training-free method that leverages pre-trained text-to-image adapters~\cite{mou2023t2i}. 
\paragraph{T2I-Adapters.} T2I-adapters enhance the capabilities of SD~\cite{rombach2022high} in text-to-image synthesis by enabling more precise control over input conditions such as depth maps, poses, edges, and more. It adopts the U-Net~\cite{ronneberger2015u} architecture, similar to SD, but fine-tunes its weights to accommodate specific task-related conditions. The features from T2I-adapters are added to the intermediate features of each block of the U-Net encoder. 
\paragraph{Modules.} Fig.~\ref{fig:save_zero} showcases the architecture of \textbf{SAVE-Zero-Shot}, which consists primarily of two main components: \textit{(i)} the T2I adapter and \textit{(ii)} the T2V module, utilizing an inflated U-Net derived from stable diffusion. The T2I adapters extract frame-level motion features that are added to the corresponding frame features of the U-Net encoder blocks. To ensure temporal consistency, the T2V model incorporates a frame-attention mechanism, as discussed in the main paper and depicted in Fig.~\ref{fig:save_zero}. We further highlight the functionality of various cross-frame attention methods in Fig.~\ref{fig:attn_cost} where it can be observed that cross-frame attention doesn't introduce any learnable parameters, and frame-attention is the most efficient variant of cross-frame attention. 
\paragraph{Results.} We present the qualitative results of our zero-generation mechanism in Fig.~\ref{fig:vid_zero_pose}, focusing on passing pose information frame-by-frame to the T2I pose-adapter. The simple cross-frame attention mechanism preserves cross-frame consistency while incorporating the motion information from the T2I adapter to generate a temporal coherent video. The generated videos have a consistent 
motion for various prompts with the same pose information. Fig.~\ref{fig:vid_zero_pose} also includes an instance where the model fails to generate a video of a "dancing tiger".  A \textit{failure case} has also been shown here where the model is struggling to replace the human subject with an animal, e.g. tiger, bear, etc. In this case, the motion information is not fully transferable as the tiger cannot move/dance like a human. Although the model generates a tiger-like object due to hard-to-transfer motion information the model also keeps the human subject. 
\section{Exploring Attention for Video Editing}\label{sec:attention}
In this section, we provide more details on the working principle of different attention mechanisms. The spatial self-attention mechanism capitalizes on the correlation between pixel locations in feature maps to establish similarities, while the cross-attention mechanism considers the correspondence between pixels and conditional inputs, such as text. Formally, given the latent representation $z_{i}$ of a video frame $v_i$, the spatial self-attention mechanism~\cite{vaswani2017attention}, is implemented as: 
$\mathrm{Attention}(Q,K,V)=\mathrm{Softmax}(\frac{Q K^T}{\sqrt{d}}) \cdot V$, where $Q=W^Q z_{i}$, $K=W^K z_{i}$, and $V=W^V z_{i}$. Here, $W^Q$, $W^K$, and $W^V$ denote learnable matrices that project the inputs to the query, key, and value components, respectively, and $d$ represents the output dimension of the key and query features.
In order to enhance temporal coherence for video editing purposes, the spatial self-attention mechanism needs to be extended to the spatio-temporal domain. Various options exist for the spatio-temporal attention (ST-Attn) mechanism, such as full attention and causal attention, which effectively capture spatio-temporal consistency. ~\cite{wang2023zeroshot} establishes that spatio-temporal attention is inevitable for video editing where each frame $z_{i}$ attends to all frames in the video. A bi-directional temporal-only attention can be another option to achieve temporal consistency; however, it completely disregards spatial modeling. Therefore, to achieve spatio-temporal cohesion, the query features are computed from the spatial features of the query frame, denoted as $z_i$. On the other hand, the key and value features are computed from the spatial features across all frames, from $z_1$ to $z_k$. In this setting, the query, key, and value are mathematically written as: $Q=W^Q [z_{i}]$, $K=W^K [z_{1:k}]$, and $V=W^V [z_{1:k}]$. Here, $W^Q$, $W^K$, and $W^V$ are the pre-trained projection weights in the self-attention layers.
~\cite{Phenaki,ho2022video,he2023latent} establishes that causal-attention is a relatively efficient approach for video generation where each frame $z_{i}$ attends to all previous frames $z_{1:i-1}$  in the video. However, these straightforward choices are not viable for generating videos with an increasing number of frames, as they entail high computational complexity. Specifically, when considering $k$ frames and $N$ sequences for each frame, both full attention and causal attention exhibit a computational complexity of $\mathcal{O}((kN)^2)$.

To generate a higher number of frames and mitigate the computational cost,~\cite{wu2022tune} proposed the utilization of a sparse version of the causal attention mechanism. In this approach, attention matrices are computed between the frame $z_{i}$ and the two preceding frames, $z_{1}$ and $z_{i-1}$, resulting in reduced computational complexity of $\mathcal{O}(2m(N)^2)$. Specifically, the query feature is derived from frame $z_{i}$, while the key and value features are obtained from the \textit{first} frame $z_{1}$ and the \textit{former} frame $z_{i-1}$, respectively. The attention operation $\mathrm{Attention}(Q,K,V)$ is then implemented with the query, key, and value mathematically written as: $Q=W^Q [z_{i}]$, $K=W^K [z_{1,i-1}]$, and $V=W^V [z_{1,i-1}]$.
% {\small
% $$Q=W^Q z_{v_i}, K=W^K \left[ z_{v_1}, z_{v_{i-1}} \right], V=W^V \left[ z_{v_1}, z_{v_{i-1}} \right],$$}%
% where $\left[ \cdot \right]$ represents the concatenation operation. Notably, the projection matrices $W^Q$, $W^K$, and $W^V$ are shared across both spatial and temporal dimensions. Refer to Figure~\ref{fig:our-attn} for a visual depiction of the proposed attention mechanism
% ~\cite{qi2023fatezero} propose another variant of sparse-causal attention where query, key, and value are defined as $Q=W^Q [z_{i}]$, $K=W^K [z_{1,w}]$, and $V=W^V [z_{1,w}]$, where $w=Round[k/2]$ corresponds to the middle frame. 
In our work, we further establish that simple frame attention is sufficient for DDIM inversion editing methods as the reversed latent features can capture the temporal information, and therefore attention with $Q=W^Q z_{i}$, $K=W^K z_{0}$, and $V=W^V z_{0}$ can achieve the desired editing performance. Fig~\ref{fig:attn_cost} further highlights the differences between various cross-frame attention mechanisms. We show the attention maps for both sparse-causal and frame attentions in Figure~\ref{fig:attention_effect}. Frame Attention produces similar performance as compared to sparse-causal attention with significantly less computational cost. (\textcolor{magenta}{Please see the attached PPT})

\section{Discussion and Limitations}\label{sec:discussion}
Recently, there have been several zero-shot video editing framework~\cite{qi2023fatezero, khachatryan2023text2videozero} that performs zero-shot video editing without any training. Although we present a zero-shot variation of SAVE, our work mainly deals with video editing through fine-tuning which requires more time and and compute. So, \emph{Why Do We Still Need to Fine-tune?} The answer to this question is two-fold: i) the limited capabilities of the zero-shot framework, and ii) the requirement of additional signals (pose information, optical flow, etc.). If one does not utilize external information (e.g. optical flow from a pre-trained model), the editing capabilities will be severely limited. For example, FateZero~\cite{qi2023fatezero} cannot edit the shape of a jeep car and change it to Porche without a pre-trained TAV model and Text-to-VideoZero~\cite{khachatryan2023text2videozero} requires knowledge of motion dynamics to perform video editing. In case of the unavailability of these motion dynamics, we need to learn it. That is where the fine-tuning is highly required. Therefore, for diverse and useful editing capabilities, fine-tuning the model is still superior, and the use of it in our work is well justified.  

One of the limitations of SAVE is that it still struggles whenever the video sequence is too long and irregular sequence of actions. We may need to employ additional measures to tackle such issues such as temporal upsampling, additional temporal layers, autoregressive scene action generation, etc.  
% \begin{wrapfigure}{R}{0.5\linewidth}
% %\begin{center}
% \centering
% %\hspace{-5mm}
% %\begin{minipage}{0.35\textwidth}
%     \includegraphics[width=1\linewidth,]{./figs/attn_calc_final.pdf}
% %    \end{center}
%     \caption{\footnotesize S }
% \label{fig:attn_cost}
% \end{wrapfigure}

% \newpage
