# Supplementary material for: SAVE: Spectral-Shift-Aware Adaptation of Image Diffusion Models for Text-driven Video Editing
Source: arXiv:2305.18670 source file (2023-12-01)
Supplement: Supplementary file 2 [file Supplementary.tex]

\vspace{-1.5mm}
\paragraph{DDIM Sampling and Inversion.} During inference, we apply deterministic DDIM sampling~\cite{ddim} to convert a random noise $z_T$ to a clean latent $z_0$ with the help of trained diffusion model ($\theta$):
\begin{equation}\label{eq:ddim_sampling}
\begin{split}
    z_{t-1} = \sqrt{\alpha_{t-1}}\left(\frac{z_t - \sqrt{1-\alpha_t}\epsilon_{\theta}(z_t)}{\sqrt{\alpha_t}}\right) + 
    \sqrt{1-\alpha_{t-1}}\epsilon_{\theta}(z_t), \quad t=T,\ldots,1, 
\end{split}
\end{equation}
where $\alpha_t = \prod_{i=1}^{t}(1-\beta_i)$ is a parameter for noise scheduling~\cite{ddim, ddpm}. DDIM Inversion is the reverse process of DDIM sampling where we can map a clean latent $z_0$ to a noisy latent $\hat{z}_T$:
\begin{equation}\label{eq:ddim_inversion}
\begin{split}
    \hat{z}_{t} = \sqrt{\alpha_{t}}\left(\frac{\hat{z}_{t-1} - \sqrt{1-\alpha_{t-1}}\epsilon_{\theta}(\hat{z}_{t-1})}{\sqrt{\alpha_{t-1}}}\right) + 
    \sqrt{1-\alpha_{t-1}}\epsilon_{\theta}(\hat{z}_{t-1}), \quad t=T,\ldots,1, 
\end{split}
\end{equation}
For applying DDIM inversion to a video, we invert each frame of the input video to the noise space. To reconstruct the original latent space using $\mathcal{P}$, we set the classifier-free guidance scale $s_{cfg}$ to 1.
